# Supplementary material for: SlideGen: Collaborative Multimodal Agents for Scientific Slide Generation
Source: arXiv:2512.04529 source file (2026-08-22)
Supplement: Supplementary file 1 [file 4o_4o_output_slides1.pdf]

# From Thousands to Billions: 3D Visual Language Grounding via Render-Supervised Distillation from 2D VLMs

Ang Cao, Sergio Arnaud, Oleksandr Maksymets, Jianing Yang, Ayush Jain, Ada Martin, Vincent-Pierre Berges, Paul McVay, Ruslan Partsey...

# CONTENTS

1. Motivation and Background
2. Key Contributions
3. Method Overview
4. Experiments and Datasets
5. Results and Analysis
6. Conclusion and Future Work

## 01 The Data Scarcity Challenge in 3D VLG

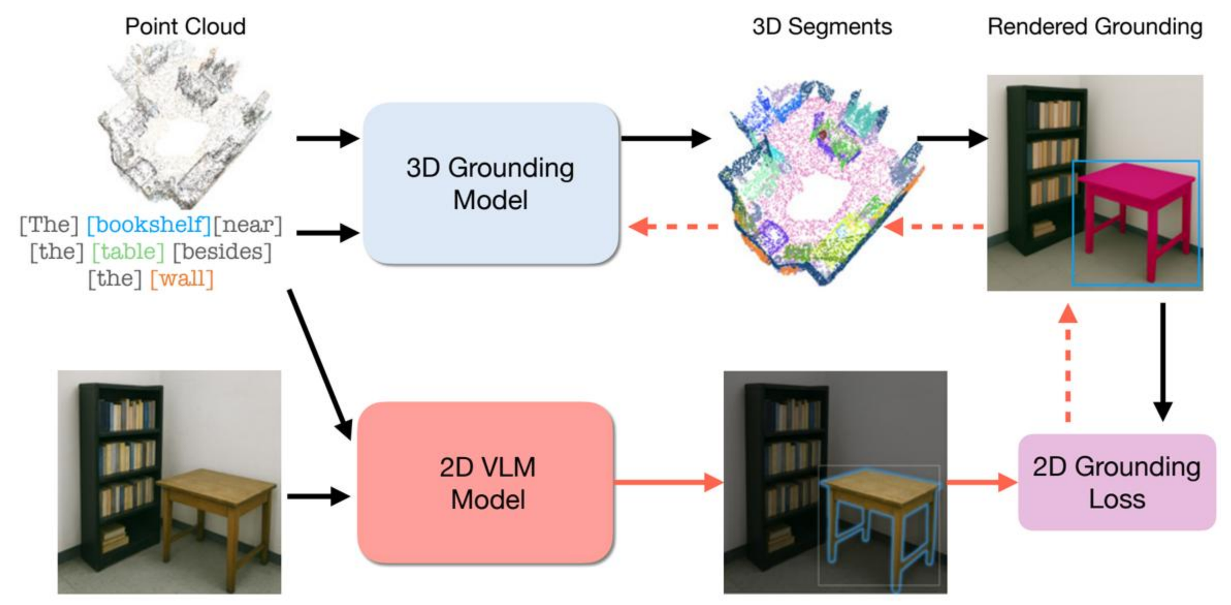


- 3D VLG faces significant data scarcity.
  - Only thousands of annotated scenes available.
  - High cost and time required for 3D annotations.
- Limits scalability and performance of 3D VLG systems.

## 01 Bridging 2D and 3D: From Lifting to Learning

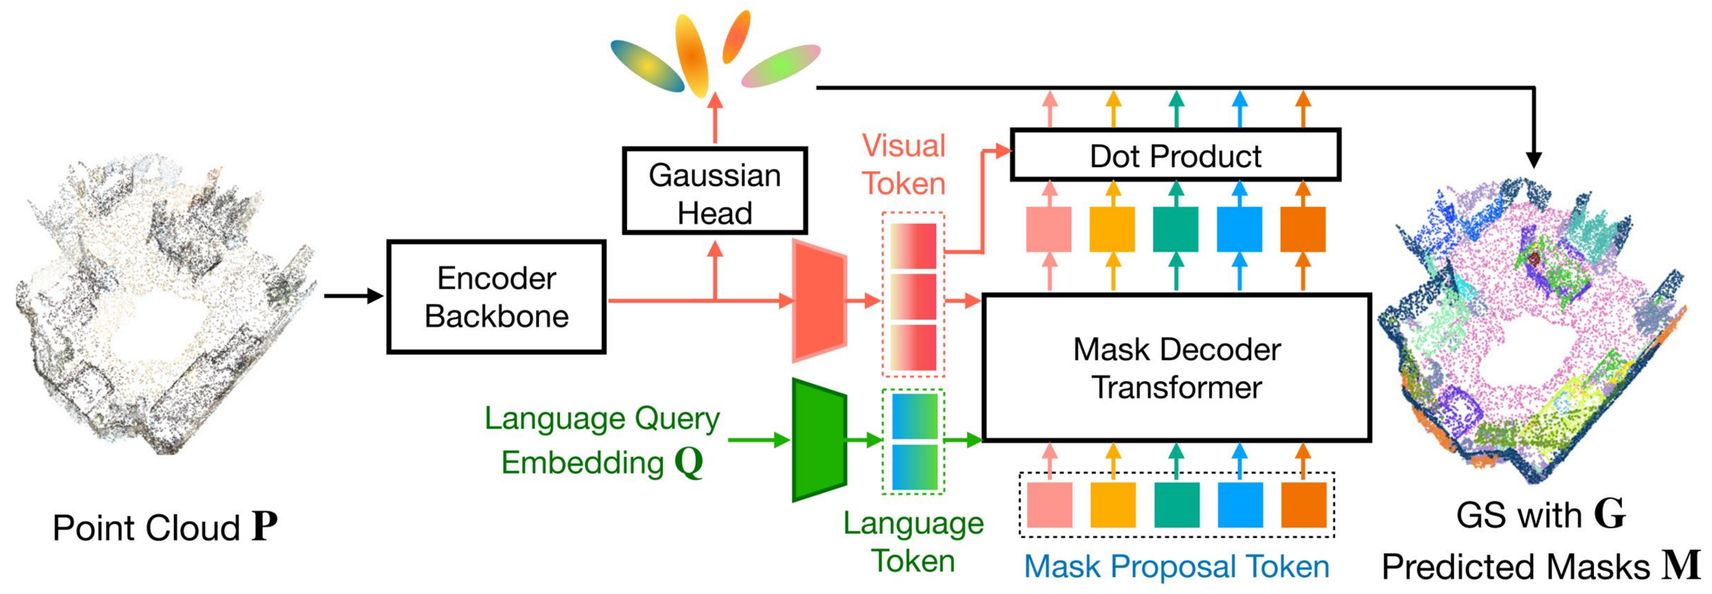


- Recent methods lift 2D models to 3D.
  - Suffer from slow optimization and accumulated errors.
  - Limited scalability.
- Differentiable rendering offers a promising alternative.
  - Enables direct training of 3D models with 2D supervision.

## 02 Render-Supervised Training Pipeline

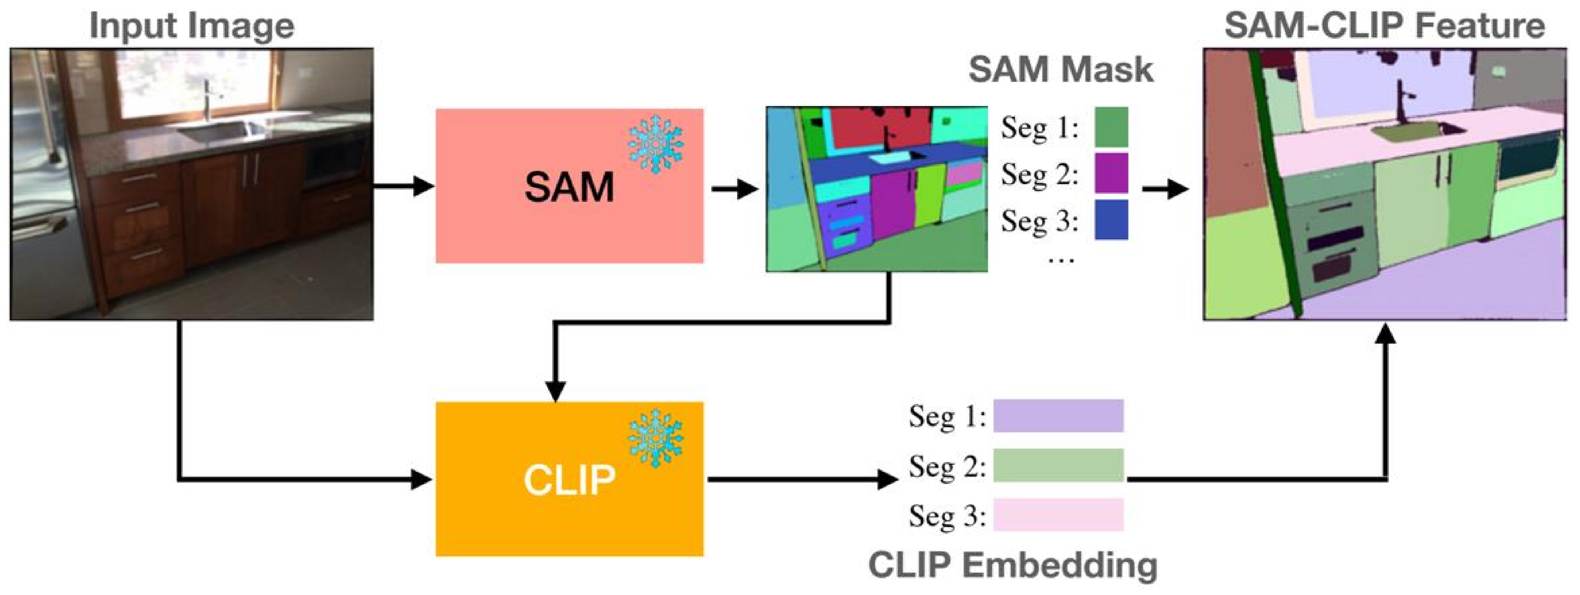


- LIFT-GS introduces a render-supervised training pipeline.
  - Requires only 2D supervision.
  - Eliminates need for scarce 3D annotations.
- Uses differentiable rendering to train 3D models with 2D losses.

## 02 Pseudo-Labeling Strategy

- Demonstrates a pseudo-labeling strategy for distilling 2D models into 3D.
  - Uses **SAM**, **CLIP**, and **LLMs**.
  - Generates 2D supervision for **3D understanding**.
- Effectively transfers internet-scale 2D knowledge into 3D.

## 03 Task Formulation

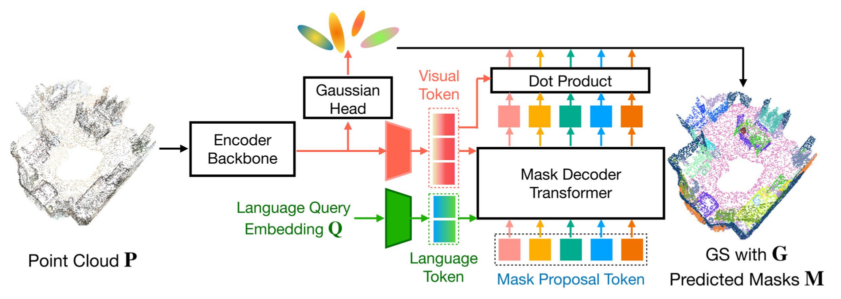


- LIFT-GS predicts **3D Gaussian representations** from **point clouds**.
  - Renders them into 2D views for supervision.
- Allows training **without 3D annotations**.
  - Leverages 2D foundation models for **pseudo-label generation**.

## 03 Losses and Architecture

| Model | $\mathcal{L}_{\text{ground}}$ | $\mathcal{L}_{\text{RGB}}$ | $\mathcal{L}_{\text{feat}}$ | Acc@0.25 | Acc@0.5 | Acc@0.75 |
|---|---|---|---|---|---|---|
| Scratch | | | | 42.19 | 27.23 | 9.66 |
| - | ✓ | | | 46.34 | 31.54 | <u>12.50</u> |
| - | ✓ | ✓ | | 46.67 | <u>31.81</u> | 12.45 |
| - | | ✓ | ✓ | **47.69** | 31.35 | 11.36 |
| - | ✓ | ✓ | ✓ | <u>47.53</u> | **33.75** | **13.49** |

$$\mathcal{L}_{\text{ground}} = \frac{1}{K}\sum_{i}^{K} \lambda_3 \mathcal{L}_{\text{mask}}(\tilde{\mathbf{M}}_{2D}^{\sigma(i)}, \mathbf{M}_{2D}^{i}) + \lambda_4 \mathcal{L}_{\text{CE}}(\mathbf{C}_{\sigma(i)}, i) \quad (3)$$

$$\sigma(i) = \arg\min_{j} \mathbf{d}_{\text{match}}(\tilde{\mathbf{M}}, \mathbf{M}_i, \mathbf{C}) \quad (4)$$

$$\mathcal{L}_{\text{RGB}} = \lambda_1 \mathcal{L}_1(I, \tilde{I}) + \lambda_2 \mathcal{L}_{\textbf{SSIM}}(I, \tilde{I}) \quad (6)$$

- Employs grounding losses and per-pixel losses.
  - Network-agnostic architecture.
  - Uses transformer-based grounding decoder.
- Gaussian decoder head predicts 3D masks and features.

8

## 04 Training Details

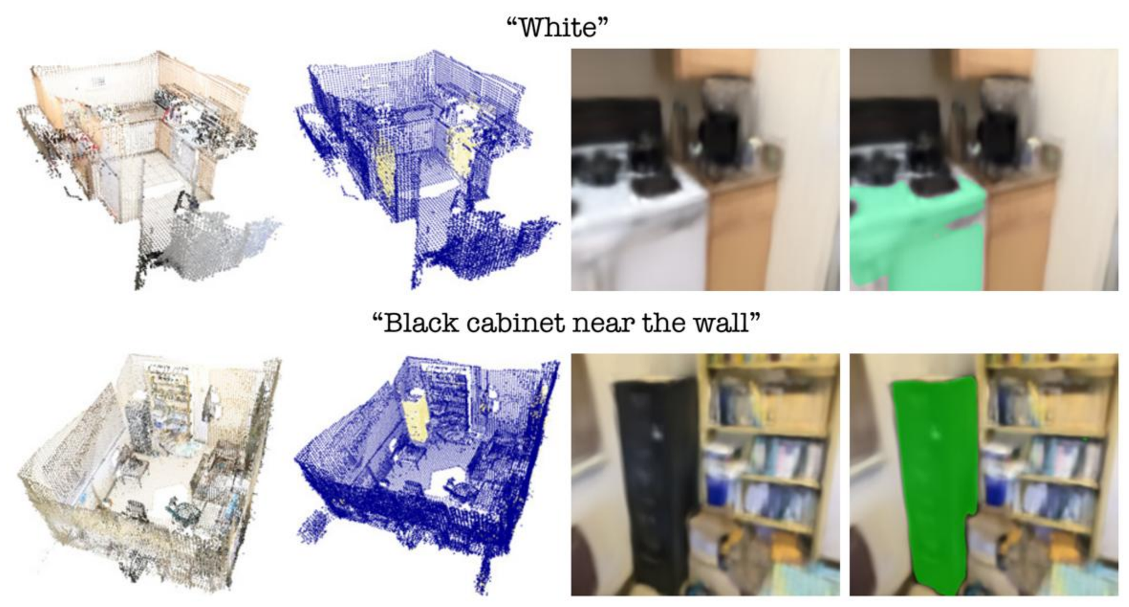


- Trained on ScanNet and other datasets.
  - Uses 2D pseudo-labels and 3D annotations.
- End-to-end optimization with differentiable rendering.
  - Various loss functions improve performance.

## 04 Evaluation on 3D Vision-Language Grounding

| Model | mAP↑ | mAP25↑ | mAP50↑ |
|---|---|---|---|
| OpenScene (Peng et al., 2023) | 11.7 | 17.8 | 15.2 |
| OpenMask3D (Takmaz et al., 2023) | 15.4 | 23.1 | 19.9 |
| PQ3D (Zhu et al., 2024) | 20.2 | 32.5 | 28.0 |
| LIFT-GS-Scratch | 22.5 | 35.1 | 30.7 |
| LIFT-GS | **25.7** | **40.2** | **35.0** |
| Δ | +3.2 ↑ | +5.1 ↑ | +4.3 ↑ |

- Evaluated on 3D open-vocabulary instance segmentation.
- Shows significant improvements over state-of-the-art methods.
  - Demonstrates effectiveness of pretraining approach.

## 05 Grounding Simple Nouns in 3D

| Model | mAP↑ | mAP25↑ | mAP50↑ |
|---|---|---|---|
| OpenScene (Peng et al., 2023) | 11.7 | 17.8 | 15.2 |
| OpenMask3D (Takmaz et al., 2023) | 15.4 | 23.1 | 19.9 |
| PQ3D (Zhu et al., 2024) | 20.2 | 32.5 | 28.0 |
| LIFT-GS-Scratch | 22.5 | 35.1 | 30.7 |
| LIFT-GS | **25.7** | **40.2** | **35.0** |
| Δ | +3.2 ↑ | +5.1 ↑ | +4.3 ↑ |

- LIFT-GS achieves substantial performance gains.
  - Outperforms state-of-the-art baselines.
- Excels in open-vocabulary 3D instance segmentation tasks.

## 05 Grounding Complex Phrases in 3D

| Method | SR3D | | NR3D | | ScanRefer | |
|---|---|---|---|---|---|---|
| | Acc@25 | Acc@50 | Acc@25 | Acc@50 | Acc@25 | Acc@50 |
| ***Mesh PC*** | | | | | | |
| LanguageRefer (Roh et al., 2021) | 39.5 | - | 28.6 | - | - | - |
| SAT-2D (Yang et al., 2021) | 35.4 | - | 31.7 | - | 44.5 | 30.1 |
| BUTD-DETR (Jain et al., 2021) | 52.1 | - | 43.3 | - | 52.2 | 39.8 |
| 3D-VisTA (Zhu et al., 2023c) | 56.5 | 51.5 | 47.7 | 42.2 | 51.0 | 46.2 |
| PQ3D (Zhu et al., 2024) | **62.0** | **55.9** | **52.2** | **45.0** | **56.7** | **51.8** |
| ***Sensor PC + Bounding Box Proposals using Mesh PC*** | | | | | | |
| 3D-VisTA (Zhu et al., 2023c) | 47.2 | 43.2 | 42.1 | 37.4 | 46.4 | 42.5 |
| ***Sensor PC*** | | | | | | |
| BUTD-DETR (Jain et al., 2021) | 43.3 | 28.9 | 32.2 | 19.4 | 42.2 | 27.9 |
| LIFT-GS-Scratch | 44.0 | 28.8 | 37.2 | 23.1 | 45.0 | 29.5 |
| LIFT-GS | **50.9** | **36.5** | **43.7** | **29.7** | **49.7** | **36.4** |
| Δ | +6.9(16%) | +7.7(27%) | +6.5(17%) | +6.6(29%) | +4.7(10%) | +6.9(23%) |

- Shows significant improvements in grounding complex phrases.
  - Achieves state-of-the-art performance in 3D referential grounding.

## 06 Conclusion and Future Work

### Conclusion

LIFT-GS addresses data scarcity in 3D VLG.

- Introduces **render-supervised distillation** from 2D VLM models.

Achieves state-of-the-art performance.

- Reveals substantial data limitations in 3D grounding.

### Future Work

Focus on improving **pseudo-labeling strategies**.

Leverage advancements in 2D foundation models.

- Enhance 3D model training and performance.

**THANKS!**
