# Supplementary material for: SlideGen: Collaborative Multimodal Agents for Scientific Slide Generation
Source: arXiv:2512.04529 source file (2026-08-22)
Supplement: Supplementary file 2 [file colorgpt5_output_slide.pdf]

# Simplex Random Features

Isaac Reid; Krzysztof Choromanski; Valerii Likhosherstov; Adrian Weller

# CONTENTS

1. Motivation And Background
2. Related Work And Orthogonality Gap
3. Key Contributions
4. Method Overview
5. Technical Details And Optimality
6. Experiments And Datasets

PART 01

## Motivation And Background

## 01 Why Random Features For Kernels?

- Random features approximate nonlinear kernels with scalable linear operations.
- IID sampling yields high-variance estimators; coupling directions reduces MSE.
- ORFs correlate directions via orthogonality; used for linear-time attention.
- PRFs and softmax/Gaussian kernels are primary targets.

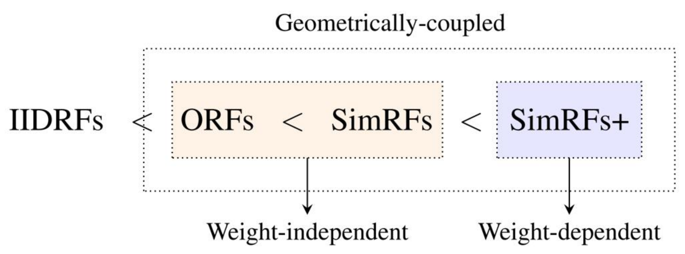


$$K(\boldsymbol{x},\boldsymbol{y}) = \mathbb{E}[\widehat{K}(\boldsymbol{x},\boldsymbol{y})], \text{ where } \widehat{K}(\boldsymbol{x},\boldsymbol{y}) \stackrel{\text{def}}{=} \phi(\boldsymbol{x})^\top \phi(\boldsymbol{y}).$$

## 01 Limitations Of Existing Mechanisms

- IID RFs have large estimator variance; ORFs reduce but may not be optimal.
- Prior theory for PRFs is asymptotic or incomplete.
- Structured couplings may not minimize pairwise resultant norms driving variance.

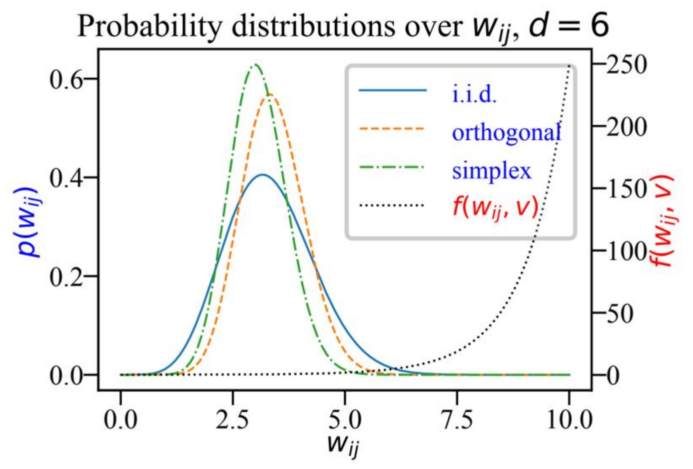


PART 02

## Related Work And Orthogonality Gap

## 02 Structured Random Features Landscape

| | Time-complexity | | |
|---|---|---|---|
| | ORFs | SimRFs | SimRFs+ |
| Regular | $\mathcal{O}(d^3)$ | $\mathcal{O}(d^3)$ | $\mathcal{O}(d^3)$ |
| Fast | $\mathcal{O}(d \log d)$ | $\mathcal{O}(d \log d)$ | $\mathcal{O}(d^3)$ |

- Structured transforms (JLT, Fastfood, HD) enable fast RFs.
- ORFs show benefits of orthogonal correlation.
- Non-asymptotic PRF forms were lacking; Performers inherit ORF suboptimality.

## 02 Orthogonality Gap Insights

- Orthogonality shrinks heavy tails of resultant sums, lowering MSE versus IID.
- A positive orthogonality gap remains; better couplings can further reduce MSE.

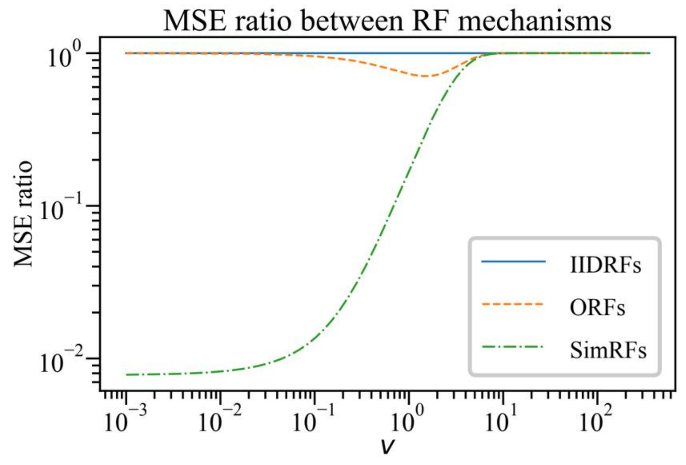


PART 03

## Key Contributions

## 03 Simplex Random Features (SimRFs)

- SimRFs align directions with a regular simplex, randomized by Haar rotations.
- Independent χ-distributed norms preserve Gaussian marginals.
- Provably minimize PRF MSE among weight-independent couplings; beat ORFs.

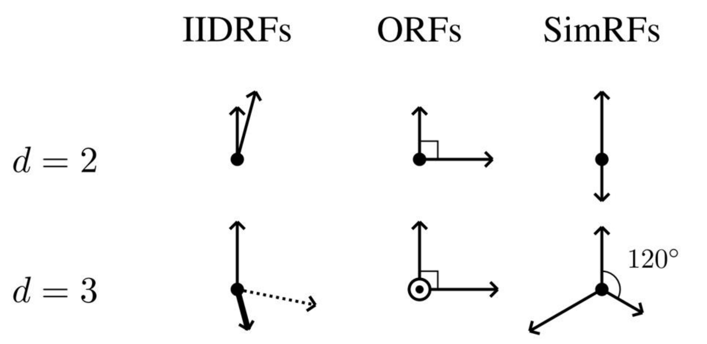


$$K_{\text{smax}}(\boldsymbol{x},\boldsymbol{y}) \stackrel{\text{def}}{=} \exp(\boldsymbol{x}^\top \boldsymbol{y}). \quad (5)$$

## 03 SimRFs+ And Theoretical Advances

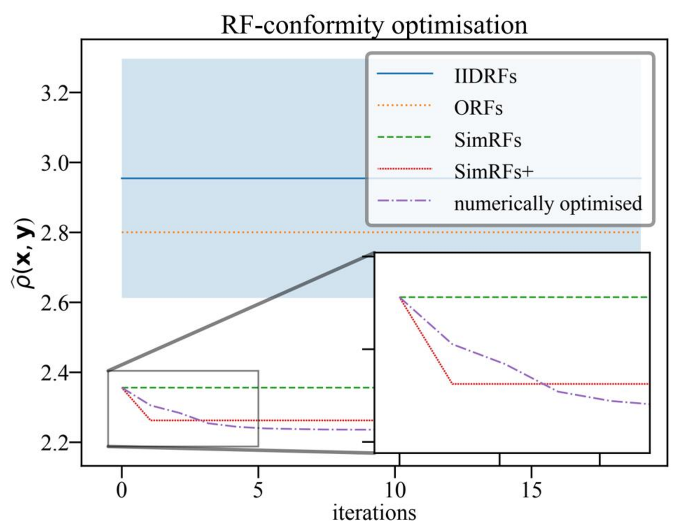


- SimRFs+ adapts angles to sampled norms; slight gains, small-v optimality.
- First non-asymptotic PRF MSE closed forms for IID, ORF, SimRF.
- Extensions to RFFs and discussion of fast implementations.

PART 04

## Method Overview

## 04 Geometrical Coupling And RF-Conformity

- Define RF-conformity ρ(x,y); estimator MSE increases with ρ.
- Geometrical coupling correlates directions with independent or dependent norms.

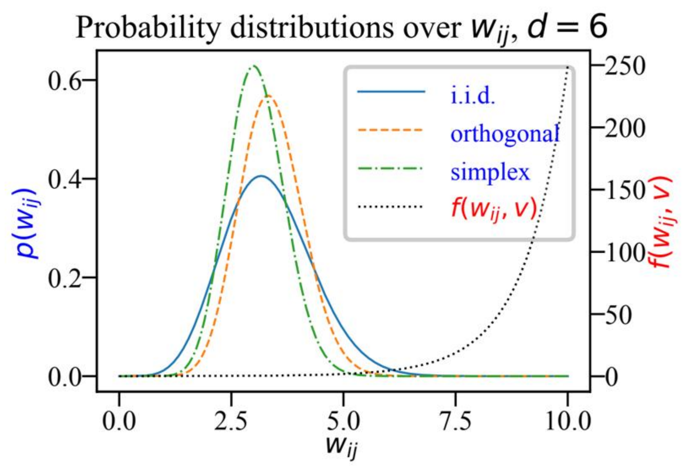


$$\text{MSE}(\widehat{K}) = \frac{e^{-2x^2-2y^2}}{m}\Big((e^{2v^2} - e^{v^2}) + (m-1)(\rho(\boldsymbol{x},\boldsymbol{y}) - e^{v^2})\Big). \quad (11)$$

## 04 Simplex Block Construction

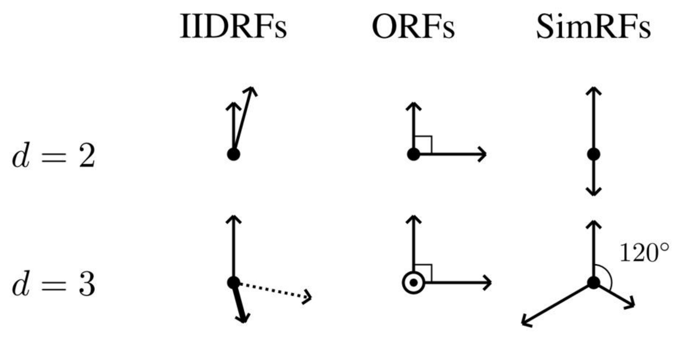


- Construct W = D S R with χ norms D, Haar orthogonal R, simplex directions S.
- Fixed obtuse angles cosθ = −1/(d−1) reduce pairwise resultants and conformity.

$$\rho(\boldsymbol{x},\boldsymbol{y}) = \frac{\Gamma(\frac{d}{2})}{m(m-1)} \sum_{i,j\neq i} \left( \sum_{k=0}^{\infty} \frac{v^{2k} w_{ij}^{2k}}{2^{2k} k! \Gamma(k+\frac{d}{2})} \right). \quad (12)$$

PART 05

## Technical Details And Optimality

## 05 Theorem: MSE Increases With RF-Conformity

- PRF estimator MSE = base term + conformity-dependent term.
- Reducing ||w_i + w_j|| lowers ρ and strictly reduces MSE.

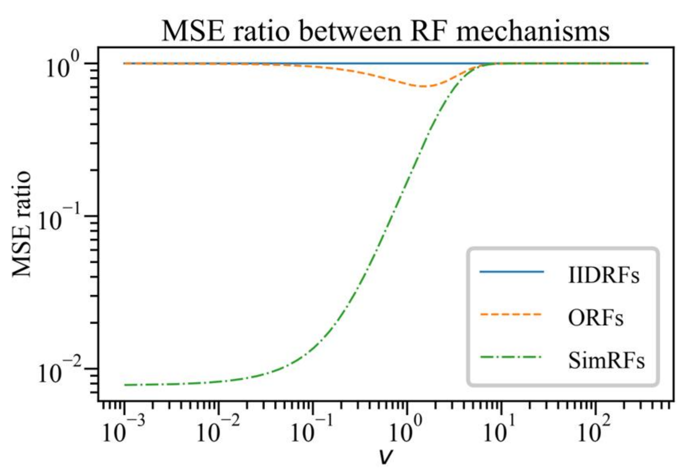


## 05 SimRFs Versus ORFs

- SimRFs enforce cosθ=−1/(d−1) vs ORF orthogonality (cosθ=0).
- Closed-form ρ enable precise non-asymptotic MSE comparisons.

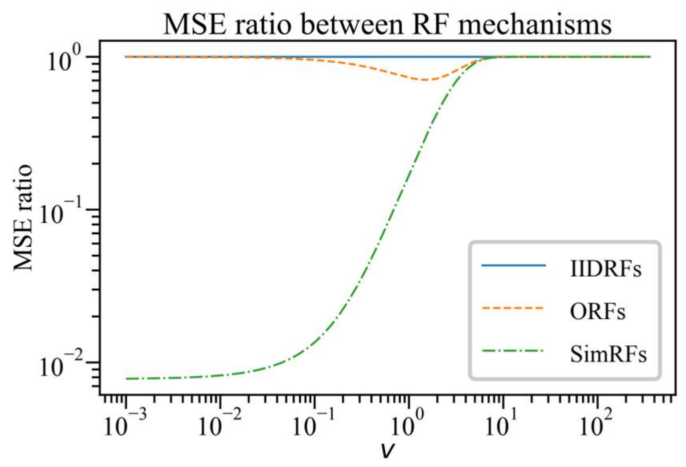


$$\frac{1}{\Gamma(\frac{d}{2})}\sum_{i,j\neq i} 1+\frac{\Gamma(\frac{d}{2})v^2\mathbb{E}(w_{ij}^2)}{4\Gamma(\frac{d}{2}+1)}\left(1+\mathcal{O}(v^2)+\ldots\right). \quad (14)$$

## 05 SimRFs+: Weight-Dependent Coupling

$$\boldsymbol{w}_i \leftarrow -\frac{\sum_{j\neq i}\boldsymbol{w}_j}{\|\sum_{j\neq i}\boldsymbol{w}_j\|_2} w_i \quad (17)$$

$$p_{i.i.d.}(w_{ij}) = \frac{w_{ij}^{d-1}e^{-w_{ij}^2/4}}{2^{d-1}\Gamma(\frac{d}{2})} \quad (18)$$

- Minimize truncated conformity; larger-norm vectors get larger angles.
- Iterative updates converge quickly from simplex initialization; gains are marginal.



## 05 Extension To RFFs And Complexity

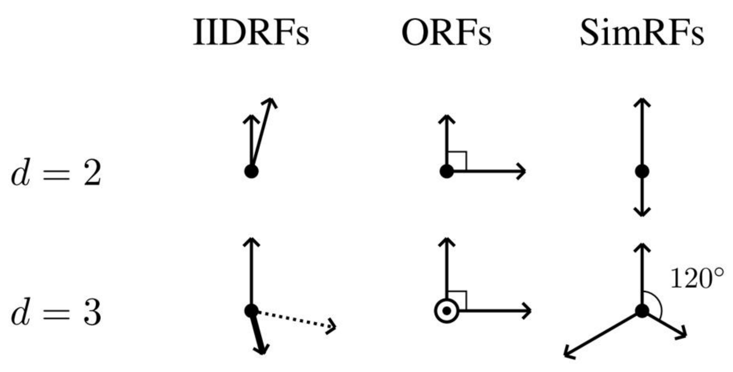


where $\boldsymbol{x}, \boldsymbol{y} \in \mathbb{R}^d$ and $v = \|\boldsymbol{x}+\boldsymbol{y}\|_2$.

- RFFs show analogous orthogonality gap; ORFs favored asymptotically.
- SimRFs use DSR with fast orthogonal proxies; SimRFs+ adds O(d^3).



PART 06

# Experiments And Datasets

## 06 Pointwise MSE And Gram Matrix Approximation

- Analytic MSE curves: SimRFs beat ORFs and IID, especially at small v.
- Gram approximation shows lower Frobenius error across feature counts.

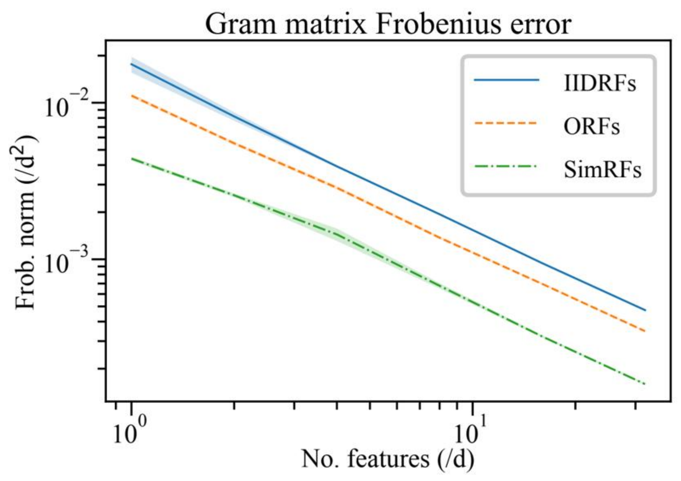


## 06 Nonparametric Classification

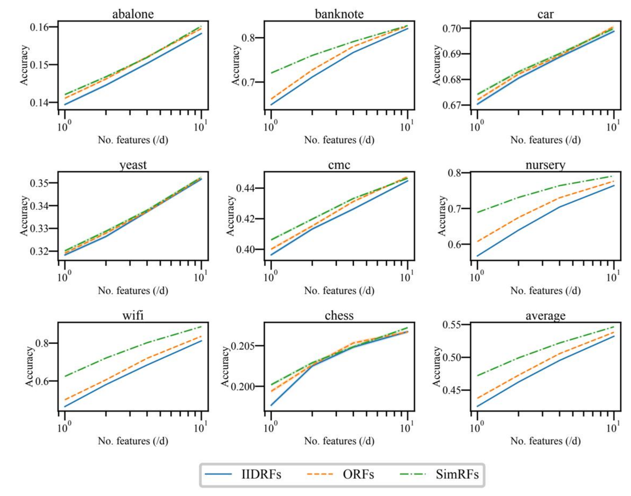


- Kernel regression: SimRFs achieve higher accuracy, converging to exact kernel.
- SimRFs+ gives minor gains in small-v regimes; σ tuned via validation.

## 06 Transformers: SimRFs-Performer

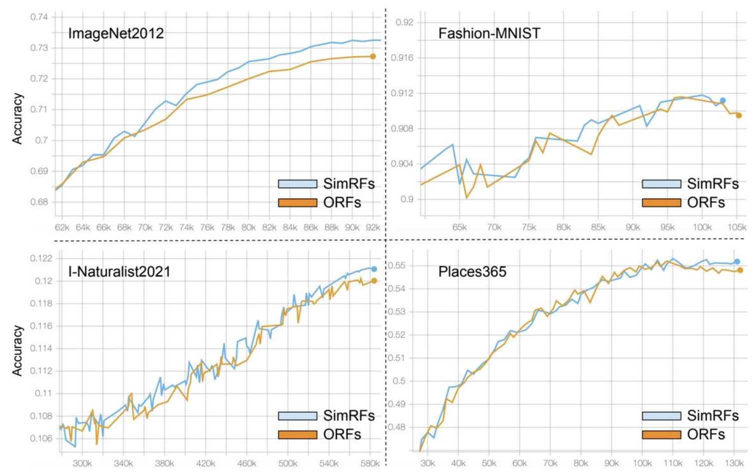


- Replacing ORFs with SimRFs in Performer improves or matches accuracy.
- Gains observed on ImageNet2012, Fashion-MNIST, iNaturalist2021, Places365.

PART 07

# Results And Analysis

## 07 Closed-Form MSE Comparisons

- Non-asymptotic closed forms quantify conformity and MSE gaps.
- Tail suppression yields hierarchy: SimRFs < ORFs < IIDRFs.

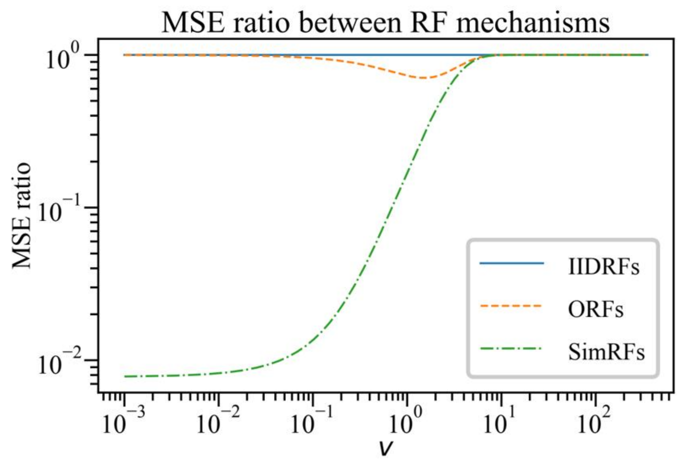


## 07 Cost And Practicality

| | Time-complexity | | |
|---|---|---|---|
| | ORFs | SimRFs | SimRFs+ |
| Regular | $\mathcal{O}(d^3)$ | $\mathcal{O}(d^3)$ | $\mathcal{O}(d^3)$ |
| Fast | $\mathcal{O}(d\log d)$ | $\mathcal{O}(d\log d)$ | $\mathcal{O}(d^3)$ |

- SimRFs are near drop-in replacements for ORFs with similar cost.
- Structured orthogonal proxies keep accuracy while reducing matvec cost.
- SimRFs+ adds overhead with marginal returns.

PART 08

# Conclusion And Future Work

## 08 Main Takeaways

- SimRFs optimally minimize PRF MSE among weight-independent couplings.
- They strictly outperform ORFs without added cost; SimRFs+ offers slight gains.
- Empirical results corroborate theory across tasks.

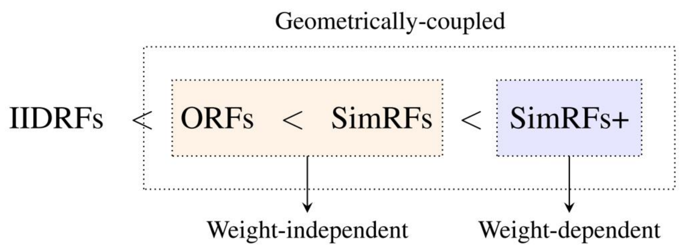


# THANKS!
