# Supplementary material for: SlideGen: Collaborative Multimodal Agents for Scientific Slide Generation
Source: arXiv:2512.04529 source file (2026-08-22)
Supplement: Supplementary file 3 [file gpt-5_gpt-5_output_slides3.pdf]

# Denoising MCMC for Accelerating Diffusion-Based Generative Models

Beomsu Kim; Jong Chul Ye

# CONTENTS

1. Motivation And Problem Formulation
2. Background On Scores, MCMC, And Diffusion
3. Key Contributions And High-Level Idea
4. Method Overview And Algorithmic Steps
5. Technical Details And Practical Choices
6. Experiments, Datasets, And Integrators

## 01 Why Accelerate Diffusion Sampling?

- **Reverse S/ODE sampling** needs hundreds–thousands of score evaluations.
- **High compute** hinders high‑ resolution, diverse generation.
- **Traditional MCMC** mixes poorly in high‑ dimensional, multimodal manifolds.
- **Goal**: faster sampling without sacrificing fidelity or diversity.

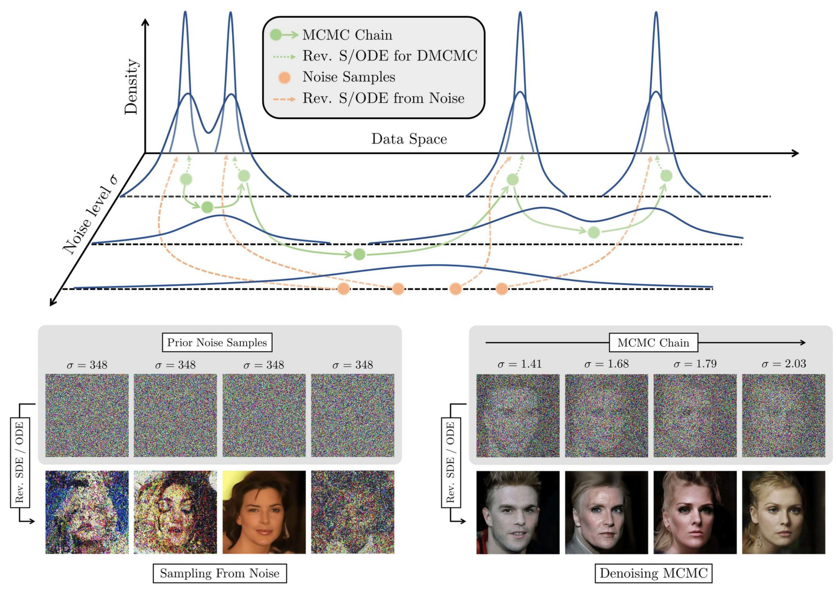


## 02 Diffusion Models, Reverse SDEs And ODEs

$$d\boldsymbol{x} = \boldsymbol{f}(\boldsymbol{x}, t)\, dt + g(t)\, d\boldsymbol{w} \qquad (2)$$

$$d\boldsymbol{x} = [\boldsymbol{f}(\boldsymbol{x}, t) - g(t)^2 \nabla_{\boldsymbol{x}} \log p_t(\boldsymbol{x})]\, dt + g(t)\, d\bar{\boldsymbol{w}} \qquad (3)$$

- Forward diffusion admits reverse SDE and probability-flow ODE.
- Integrating reverse dynamics with scores yields samples.
- VE and VP are equivalent via change-of-variables; solver choice matters.



## 03 Denoising MCMC: Product-Space Initialization

- Propose DMCMC: MCMC over (data, noise) then short reverse integration.
- Chains dwell near manifold at low noise, shortening integration interval.
- Enables faster, high-fidelity sampling under tight NFE budgets.

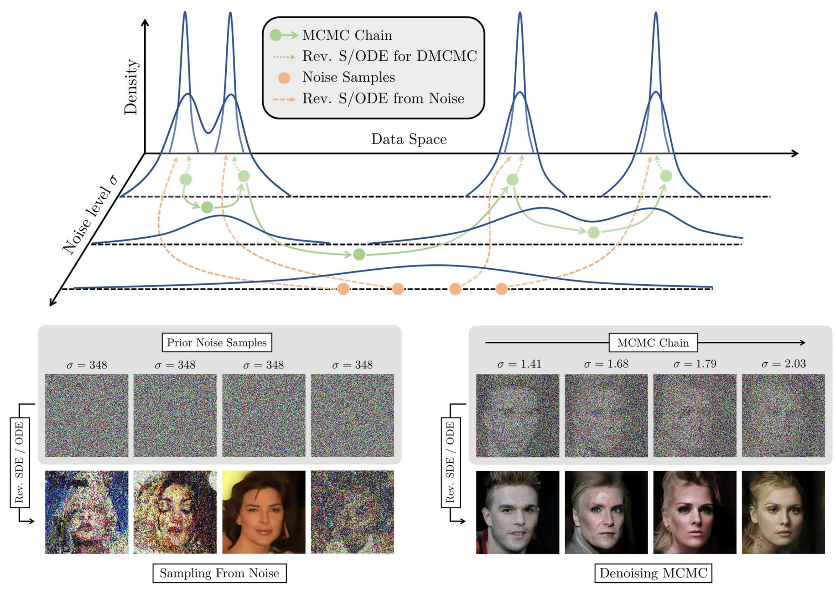


## 03 Key Contributions And High-Level Idea

### Denoising Langevin Gibbs (DLG) Instance

DLG alternates Langevin x-updates and σ-updates via classifier.

Requires pretrained score and lightweight noise-level classifier.

Compatible with any reverse S/ODE; works for VE or VP scores.

### Orthogonality To Solver Improvements

DMCMC provides better initialization, complementing solver advances.

Combining DMCMC with improved integrators further boosts performance.

Enhances predictor–corrector by strengthening initialization quality.

## 04 Step 1: MCMC On Data–Noise Product Space

$$d\boldsymbol{x} = \left[\boldsymbol{f}(\boldsymbol{x}, t) - (1/2) \cdot g(t)^2 \nabla_{\boldsymbol{x}} \log p_t(\boldsymbol{x})\right]\, dt \qquad (4)$$

$$d\boldsymbol{x} = \sqrt{\frac{d[\sigma^2(t)]}{dt}}\, d\boldsymbol{w} \qquad (5)$$

- Define joint target over data and noise with smoothing and prior.
- MCMC samples (x, σ), moving up for mixing and down near manifold.
- Prior can bias toward small σ while preserving mixing.

## 04 DLG: Alternating Langevin And Noise Prediction

- Langevin step uses conditional score at current σ.
- Predict next σ via classifier approximating p(σ|x).
- Select lowest‑ σ state per block for denoising.

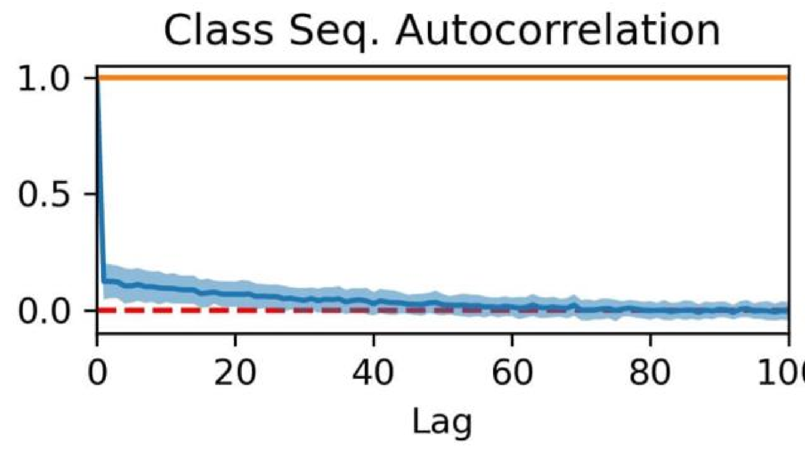


$$\hat{p}(\boldsymbol{x} \mid \sigma) := \int p_\sigma(\boldsymbol{x} \mid \tilde{\boldsymbol{x}}) p(\tilde{\boldsymbol{x}})\, d\tilde{\boldsymbol{x}}. \qquad (7)$$



## 05 Technical Details And Practical Choices

### Warm Starts, Skipping, And Selection

Warm start: generate clean, add noise, run few Gibbs updates.

Reduce autocorrelation by processing every n_skip-th block.

Within blocks, pick minimum‑ σ state for denoising.

Allocate NFEs between chain and denoising for balance.

### Choice Of Prior And Hyperparameters

Use 1/σ prior to nudge toward low noise while mixing.

Overly sharp priors slow convergence; trade-offs exist.

Tune step size η and denoising NFE ratio jointly.

## 06 Mixing And Mode Coverage

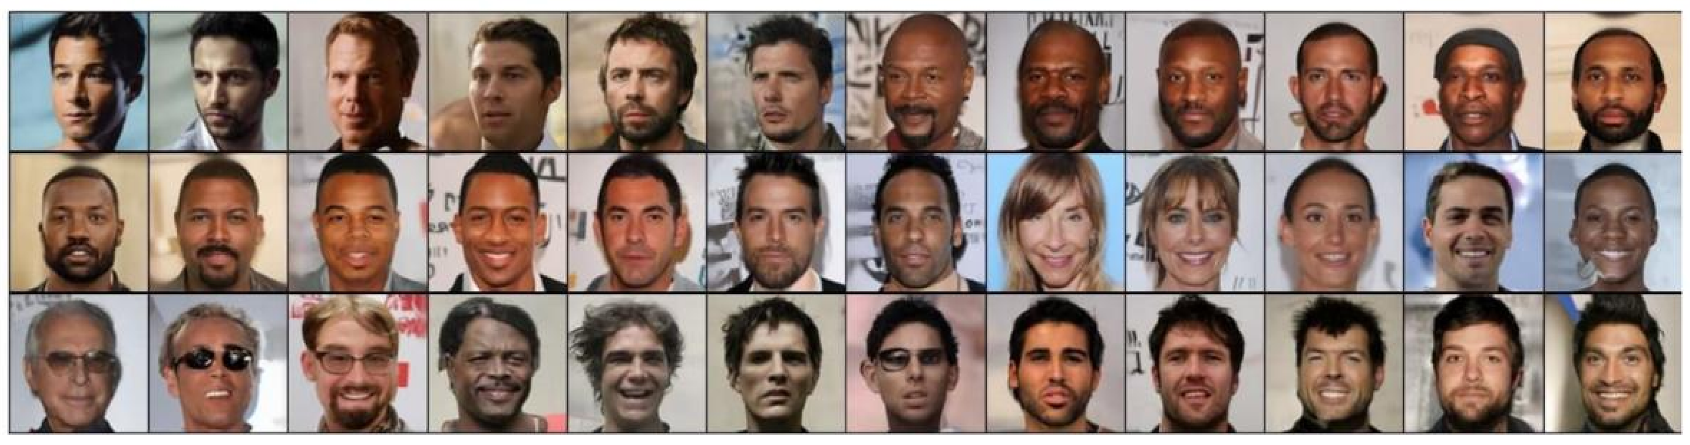

- DLG traverses modes in 1k‑ mode MoG and matches class statistics.
- CelebA‑ HQ chains show smooth attribute transitions with quality intact.
- Autocorrelation analyses confirm improved mixing.

## 06 Image Generation Benchmarks

- DLG accelerates multiple samplers across CIFAR-10, CelebA-HQ, FFHQ.
- Reduces NFEs needed for competitive or better FID.
- Works for deterministic and stochastic integrators.

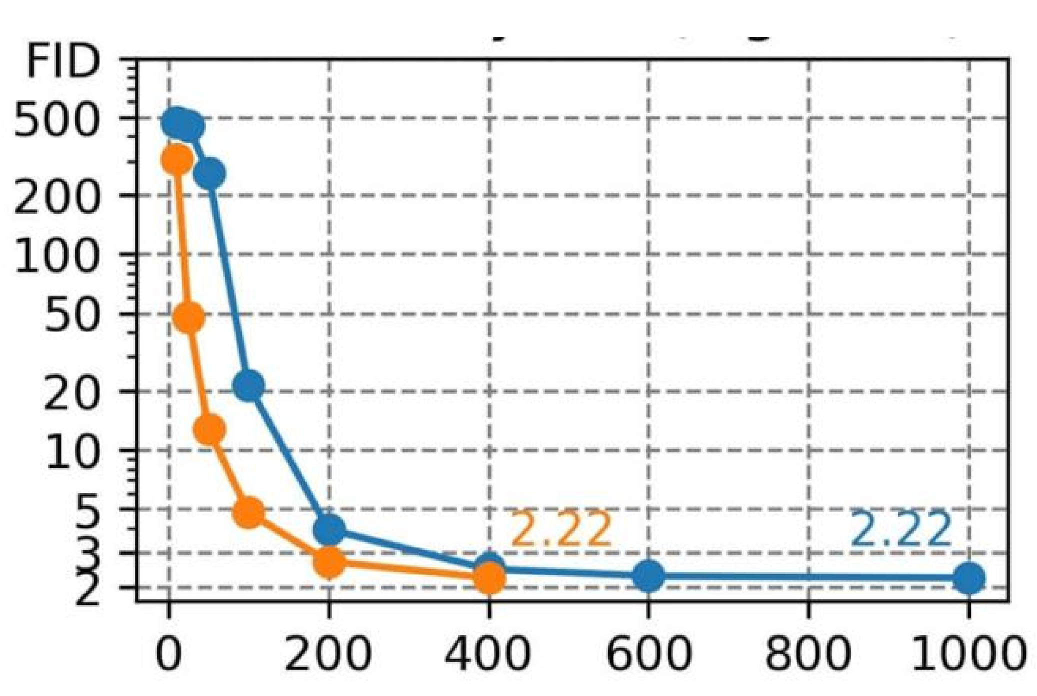


## 06 Conditional Generation And Scores

| Class | 0 | 1 | 2 | 3 | 4 | 5 | 6 | 7 | 8 | 9 |
|---|---|---|---|---|---|---|---|---|---|---|
| No DLG | 14.3 | 11.6 | 15.8 | 17.7 | 14.7 | 16.9 | 16.0 | 13.4 | 11.1 | 11.3 |
| WIth DLG | 12.2 | 9.3 | 13.5 | 14.8 | 11.6 | 13.6 | 12.7 | 10.6 | 9.3 | 8.5 |

- DLG improves class-conditional generation with VE and VP scores.
- Per-class FID improves when adding DLG to same integrator.

## 07 State-Of-The-Art In Low-NFE Regime

| Method | NFE 10 | NFE 20 | NFE 50 |
|---|---|---|---|
| DPM-Solver-2 (VP) | 5.28 (+2 NFE) | 3.02 (+4 NFE) | 2.69 (−2 NFE) |
| DPM-Solver-3 (VP) | 6.03 (+2 NFE) | 2.75 (+4 NFE) | 2.65 (−2 NFE) |
| DEIS (VP) | 4.17 (+0 NFE) | 2.86 (+0 NFE) | 2.57 (+0 NFE) |
| DEIS (VE) | 20.89 (+0 NFE) | 16.59 (+0 NFE) | 16.31 (+0 NFE) |
| KAR1 (VP) | 9.70 (+1 NFE) | 3.23 (+5 NFE) | 2.97 (+1 NFE) |
| KAR1 (VE) | 14.12 (+1 NFE) | 4.46 (+5 NFE) | 4.1 (+1 NFE) |
| DLG+KAR1 (VP) | **3.25** (+0.1 NFE) | **2.49** (−3.9 NFE) | 2.49 (−33.9 NFE) |
| DLG+KAR1 (VE) | 3.86 (+0.1 NFE) | 2.63 (+0.1 NFE) | **2.45** (−0.9 NFE) |

- DLG+KAR1 achieves SOTA FID at ~10–16 NFE on CIFAR-10.
- CelebA-HQ-256: DLG+KAR2 outperforms prior 4000-NFE results.
- FFHQ-1024 shows large low-NFE FID gains.

## 07 Ablations: η, NFE Split, And Necessity Of Denoising

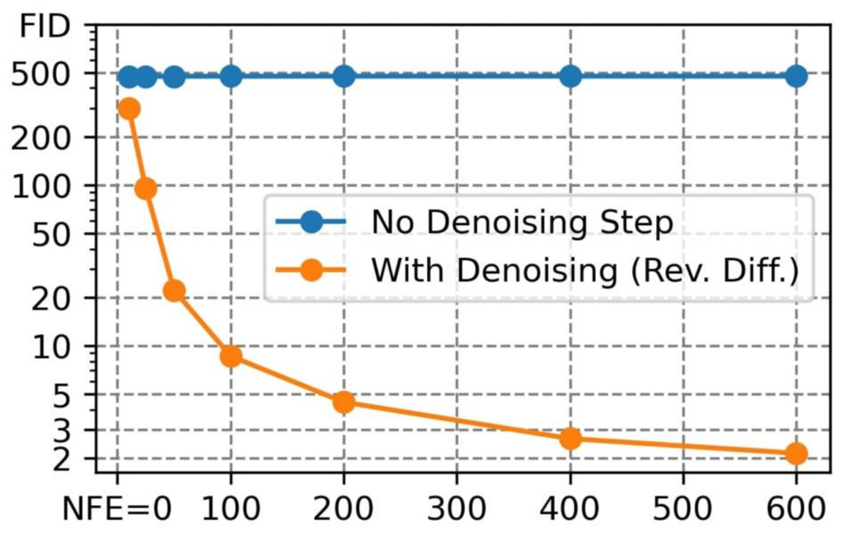


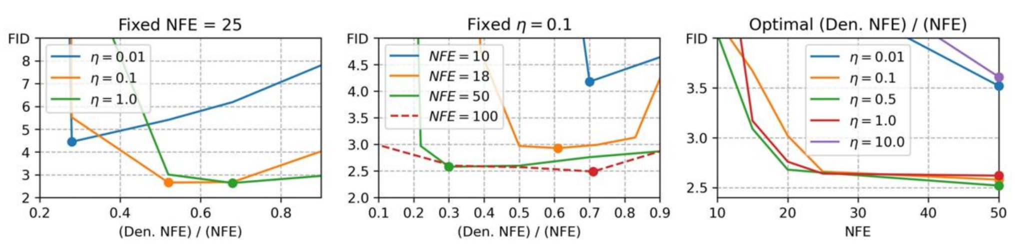


- Optimal η and denoising-to-total NFE ratio balance diversity and quality.
- As NFE grows, near-optimal ratios widen.
- Removing denoising collapses quality—denoising is essential.

## 07 σ-Trajectory And Manifold Proximity

- σ trajectories move up/down, enabling mode transitions.
- Predicted σ correlates with distance-to-manifold scaling.
- Classifier keeps chains where score gradients are informative.

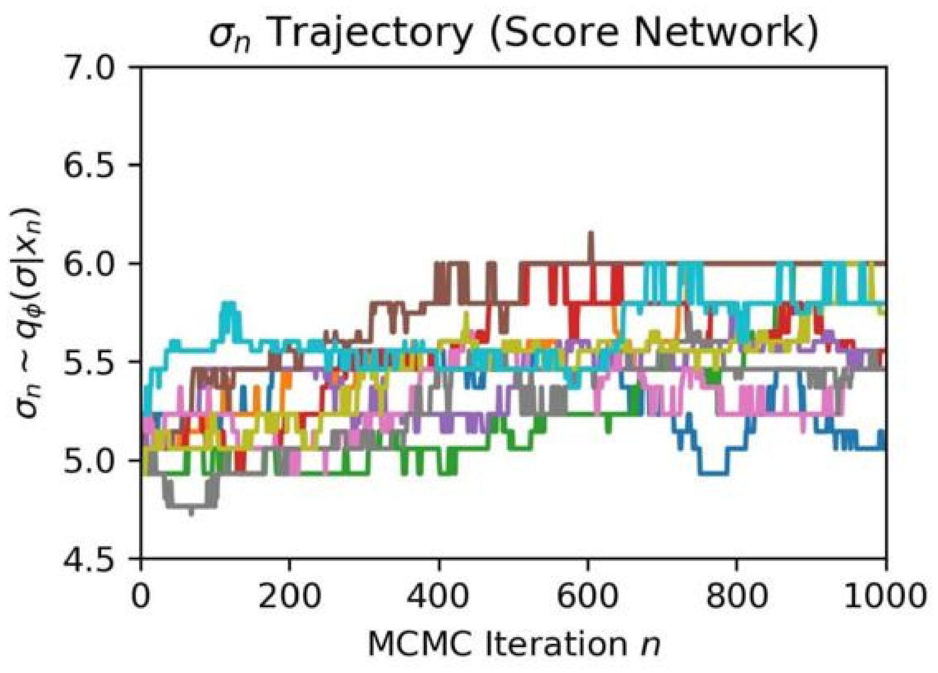


## 08 Relation To Predictor-Corrector And Distillation

- DMCMC complements PC by improving initialization; accelerates PC pipelines.
- Compared to distillation, requires far less extra training compute.
- Achieves competitive FID at similar NFE with minimal overhead.

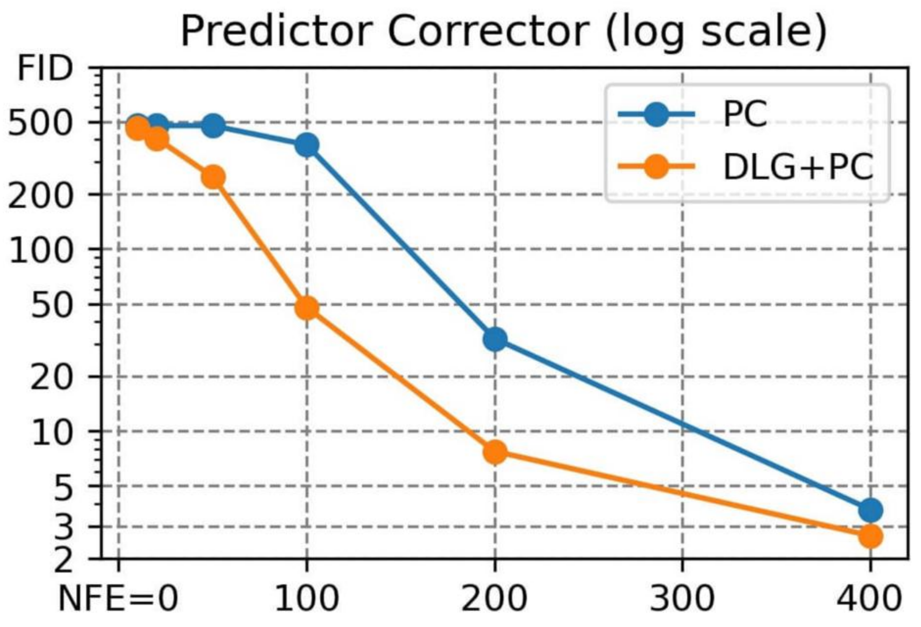


## 08 Related Work, Limitations, And Impact

### Limitations And Future Extensions

Extensions to guided diffusion (classifier/CLIP) are natural next steps.

Further theory on Langevin Gibbs convergence and adaptive priors needed.

Trade-offs between stability and speed warrant deeper analysis.

### Societal Impacts And Reproducibility

Acceleration reduces compute and energy for generative models.

Faster sampling can amplify misuse risks; responsible deployment is needed.

Code and checkpoints provided with clear hyperparameters and pseudocode.

## 09 Main Takeaways

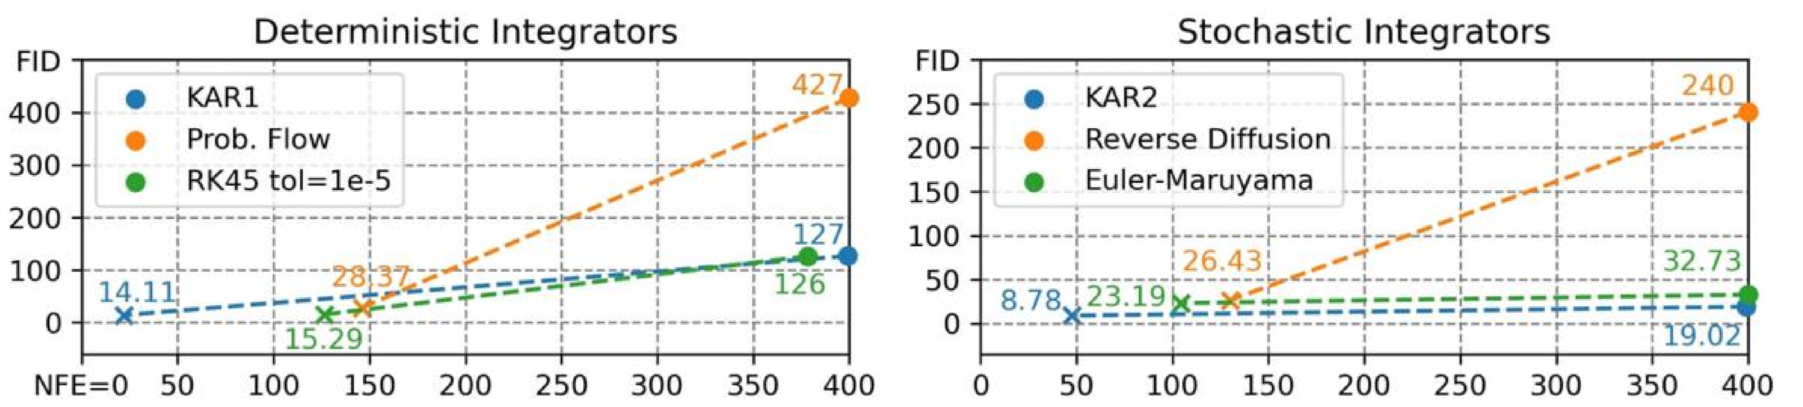


- DMCMC samples in **data–time space** first, then denoises, shortening integration.
- DLG is simple, plug-and-play, and scales to high resolution.
- Delivers state-of-the-art results in low-NFE regimes.
