# Supplementary material for: SlideGen: Collaborative Multimodal Agents for Scientific Slide Generation
Source: arXiv:2512.04529 source file (2026-08-22)
Supplement: Supplementary file 4 [file notes.pdf]

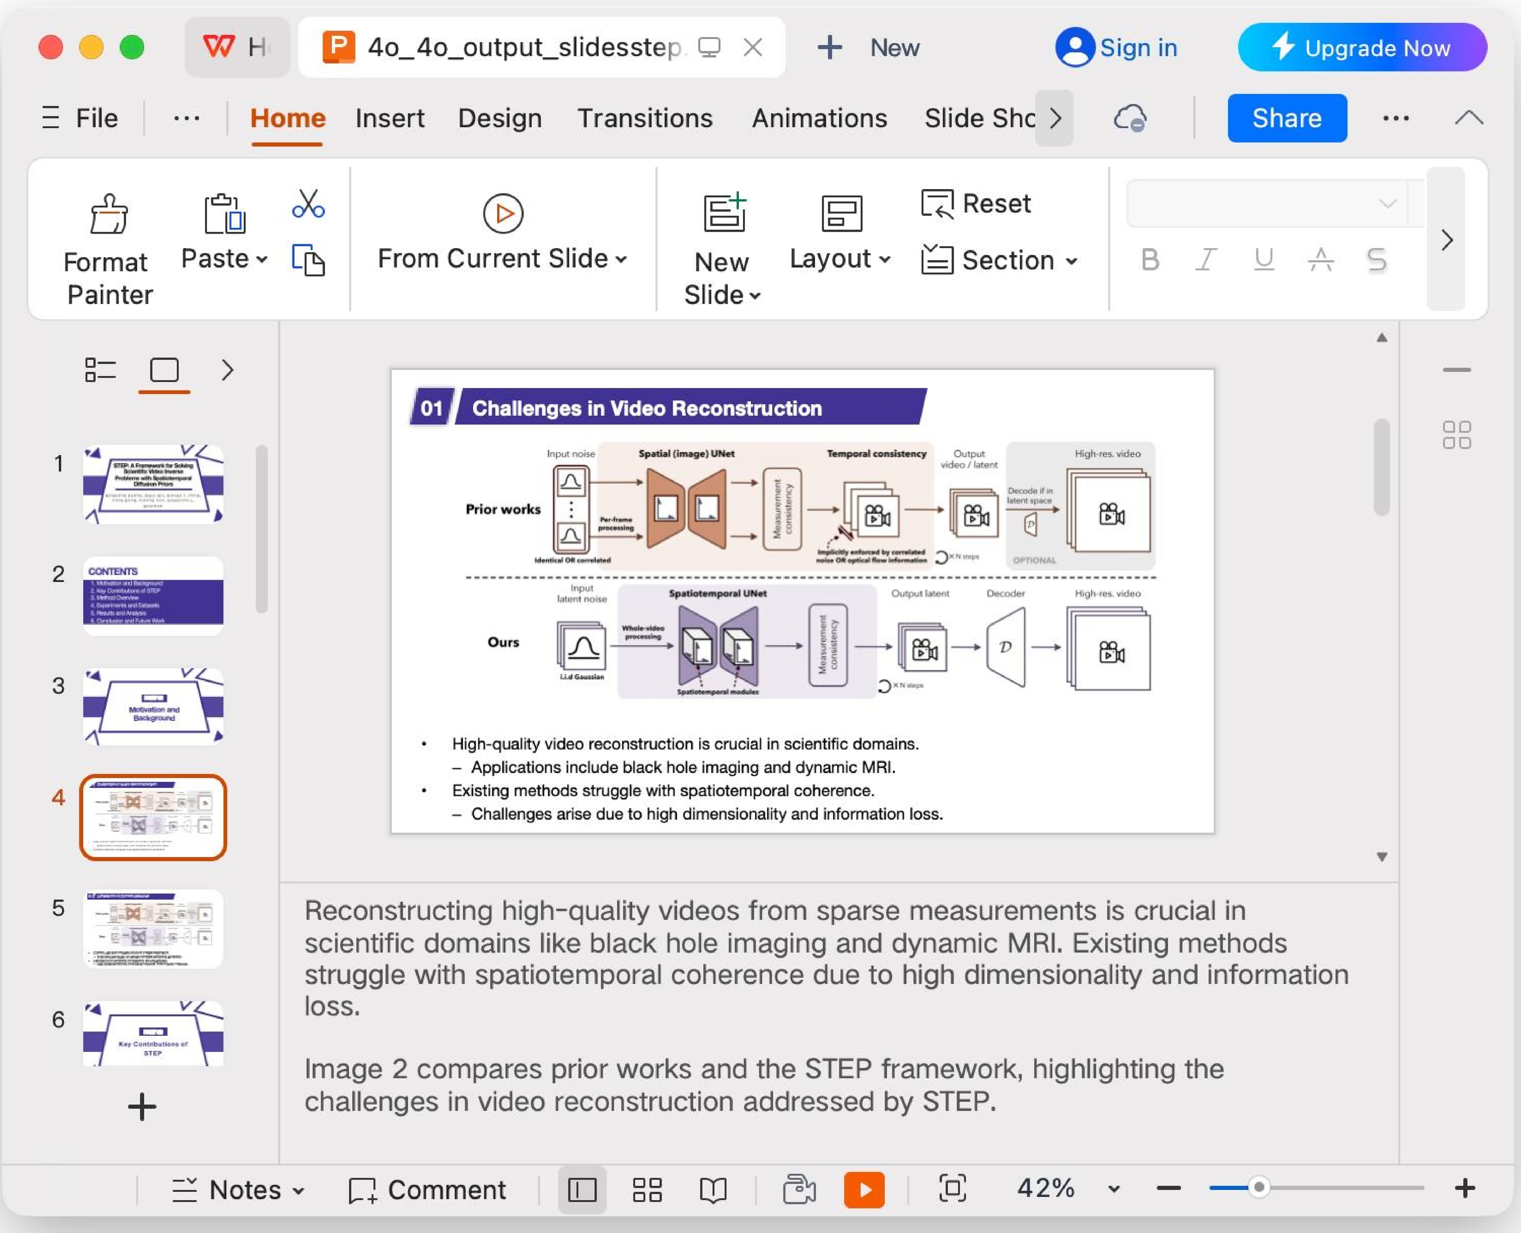
4o_4o_output_slidesstep
01 Challenges in Video Reconstruction
High-quality video reconstruction is crucial in scientific domains.
– Applications include black hole imaging and dynamic MRI.
Existing methods struggle with spatiotemporal coherence.
– Challenges arise due to high dimensionality and information loss.
Reconstructing high-quality videos from sparse measurements is crucial in scientific domains like black hole imaging and dynamic MRI. Existing methods struggle with spatiotemporal coherence due to high dimensionality and information loss.
Image 2 compares prior works and the STEP framework, highlighting the challenges in video reconstruction addressed by STEP.

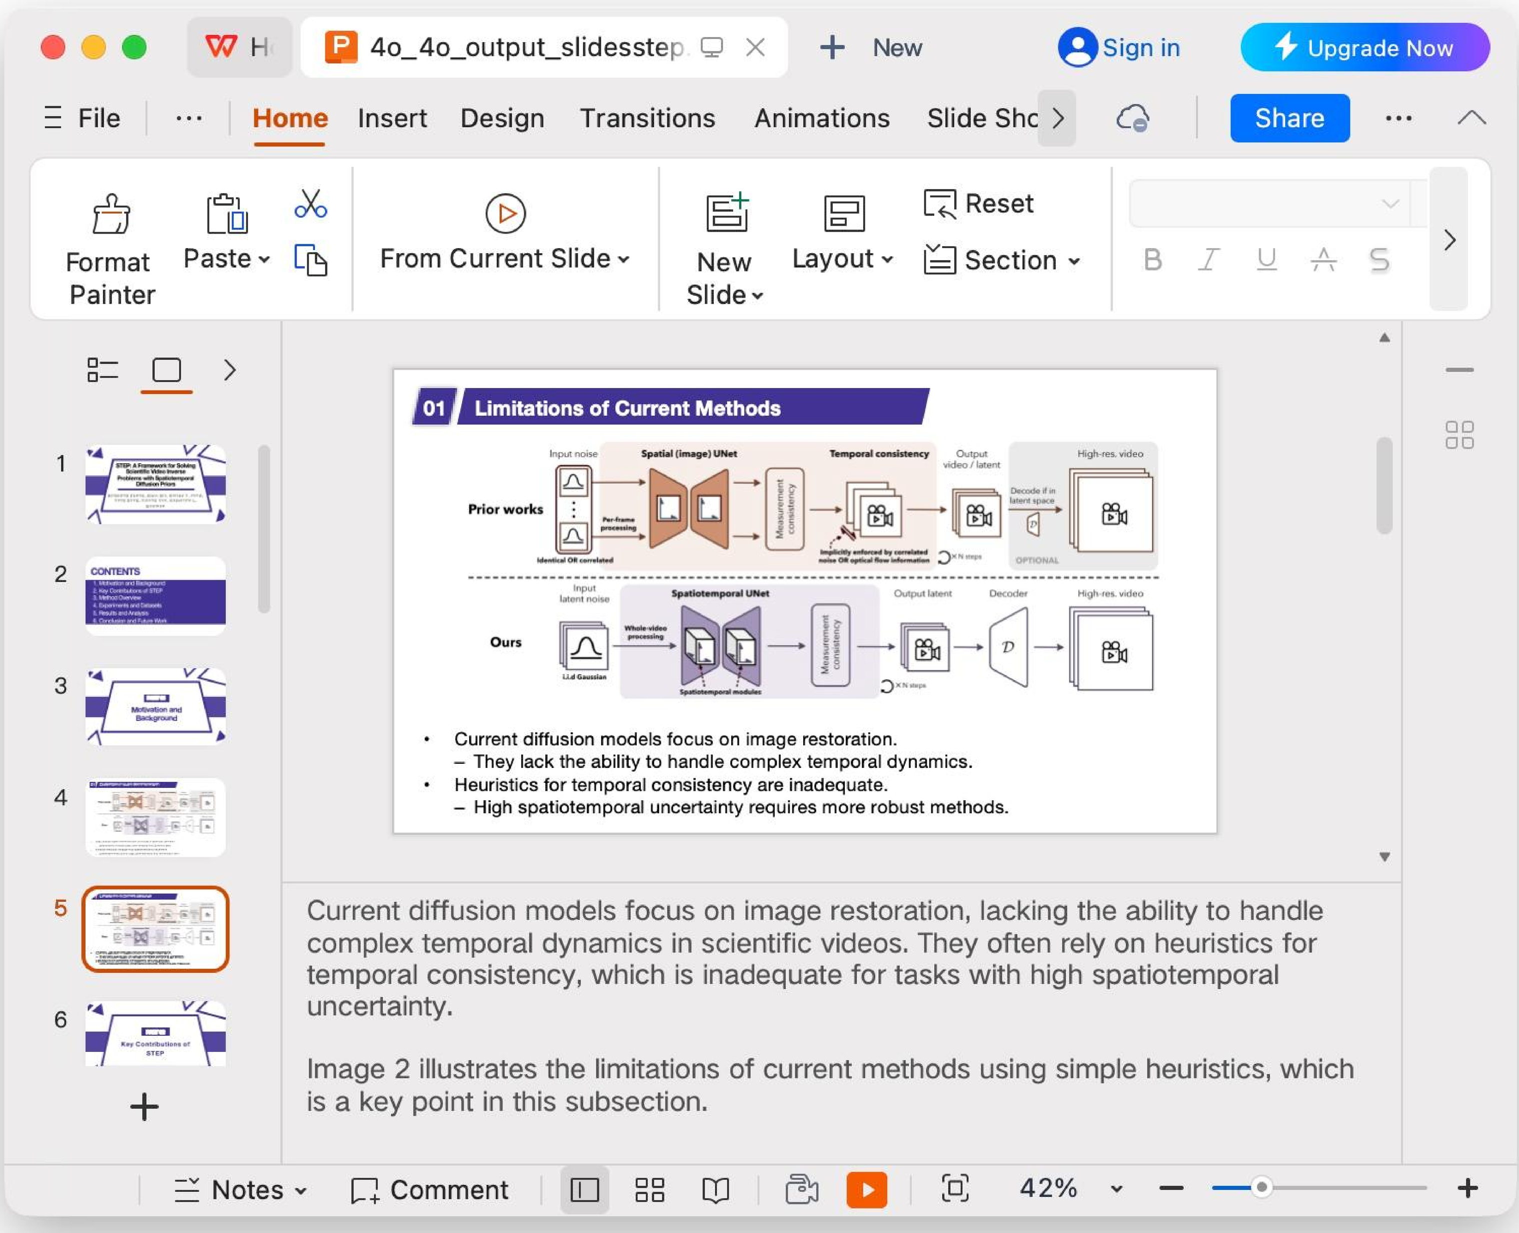
4o_4o_output_slidesstep
01 Limitations of Current Methods
Current diffusion models focus on image restoration.
– They lack the ability to handle complex temporal dynamics.
Heuristics for temporal consistency are inadequate.
– High spatiotemporal uncertainty requires more robust methods.
Current diffusion models focus on image restoration, lacking the ability to handle complex temporal dynamics in scientific videos. They often rely on heuristics for temporal consistency, which is inadequate for tasks with high spatiotemporal uncertainty.
Image 2 illustrates the limitations of current methods using simple heuristics, which is a key point in this subsection.

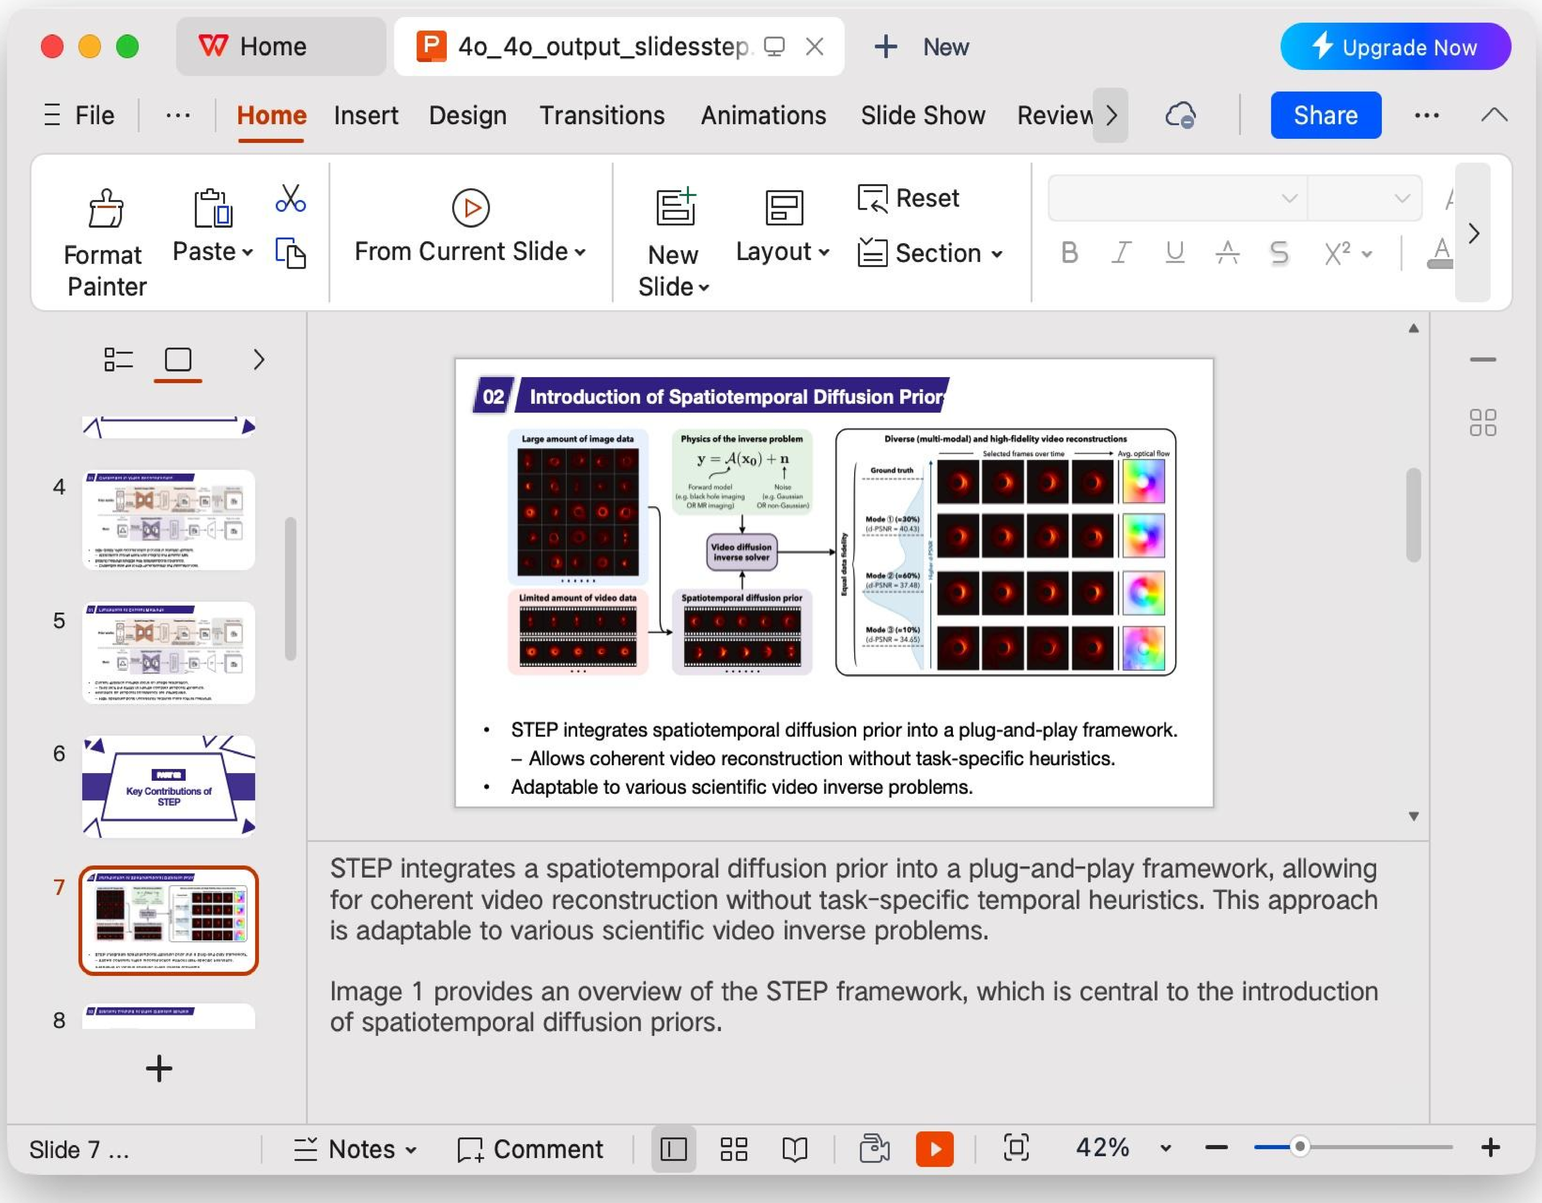
4o_4o_output_slidesstep
02 Introduction of Spatiotemporal Diffusion Prior
STEP integrates a spatiotemporal diffusion prior into a plug-and-play framework.
– Allows coherent video reconstruction without task-specific heuristics.
Adaptable to various scientific video inverse problems.
STEP integrates a spatiotemporal diffusion prior into a plug-and-play framework, allowing for coherent video reconstruction without task-specific temporal heuristics. This approach is adaptable to various scientific video inverse problems.
Image 1 provides an overview of the STEP framework, which is central to the introduction of spatiotemporal diffusion priors.

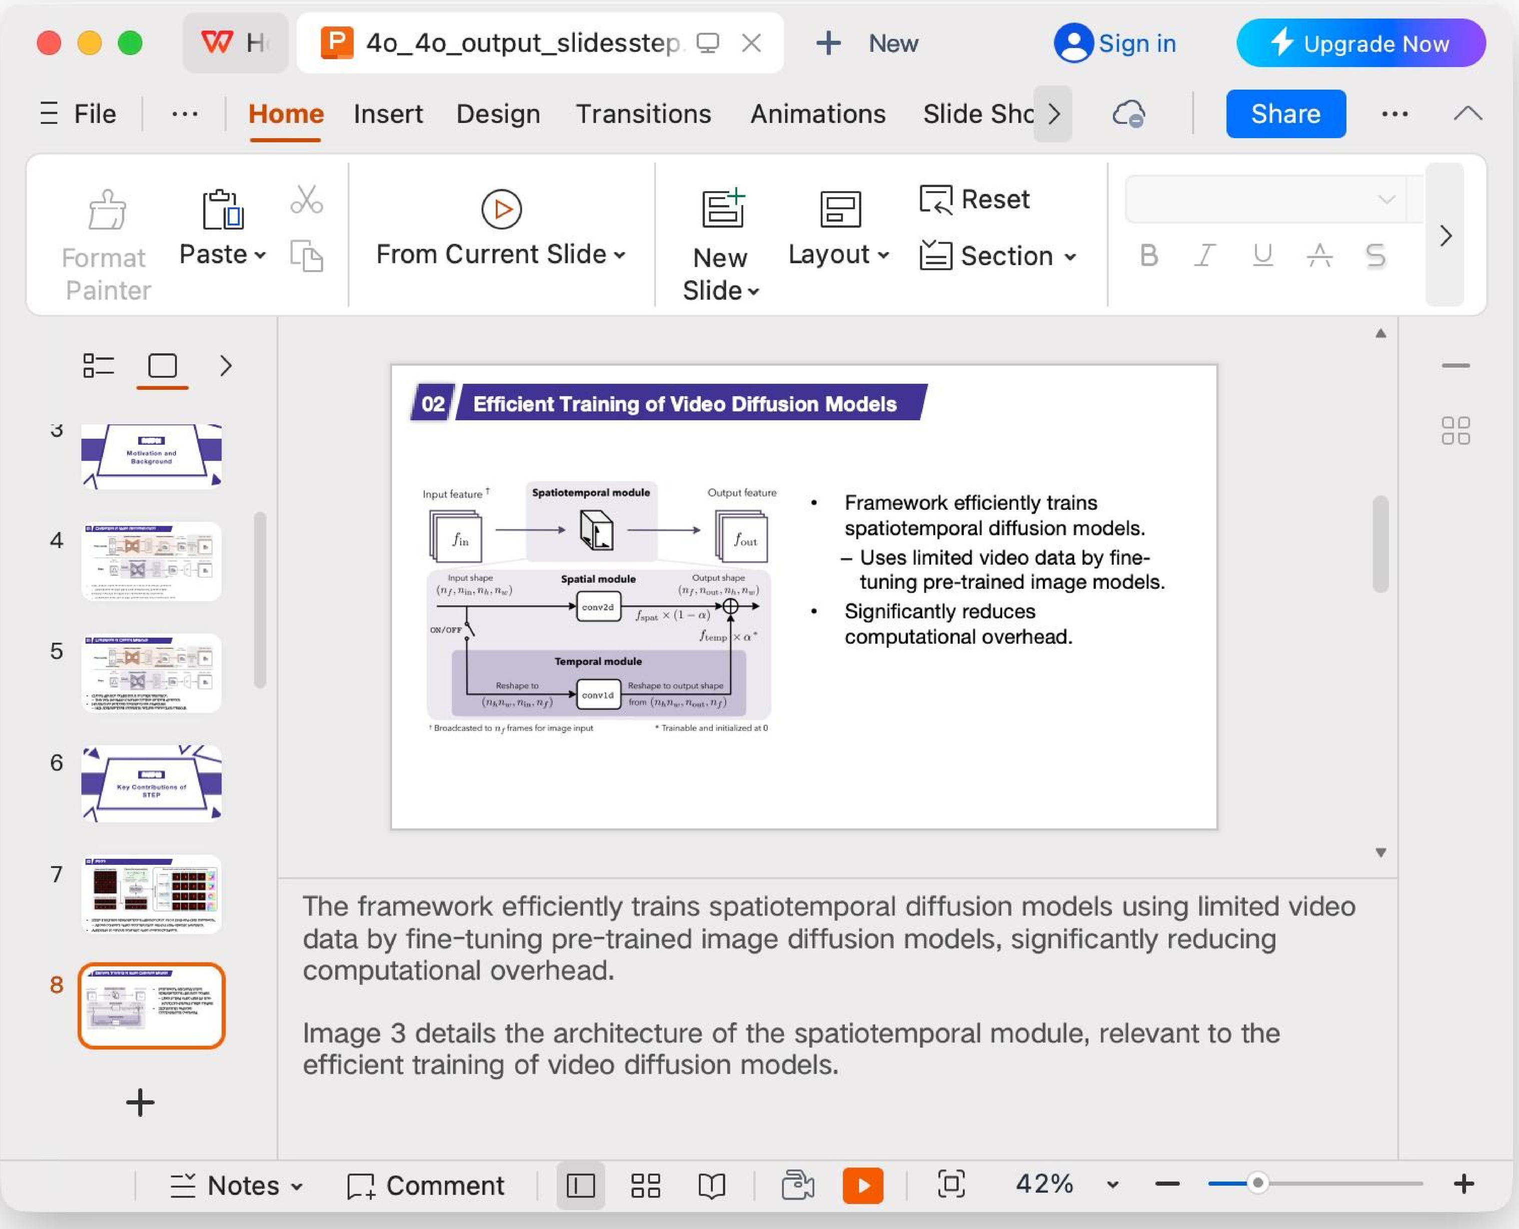
4o_4o_output_slidesstep
02 Efficient Training of Video Diffusion Models
Framework efficiently trains spatiotemporal diffusion models.
– Uses limited video data by fine-tuning pre-trained image models.
Significantly reduces computational overhead.
The framework efficiently trains spatiotemporal diffusion models using limited video data by fine-tuning pre-trained image diffusion models, significantly reducing computational overhead.
Image 3 details the architecture of the spatiotemporal module, relevant to the efficient training of video diffusion models.

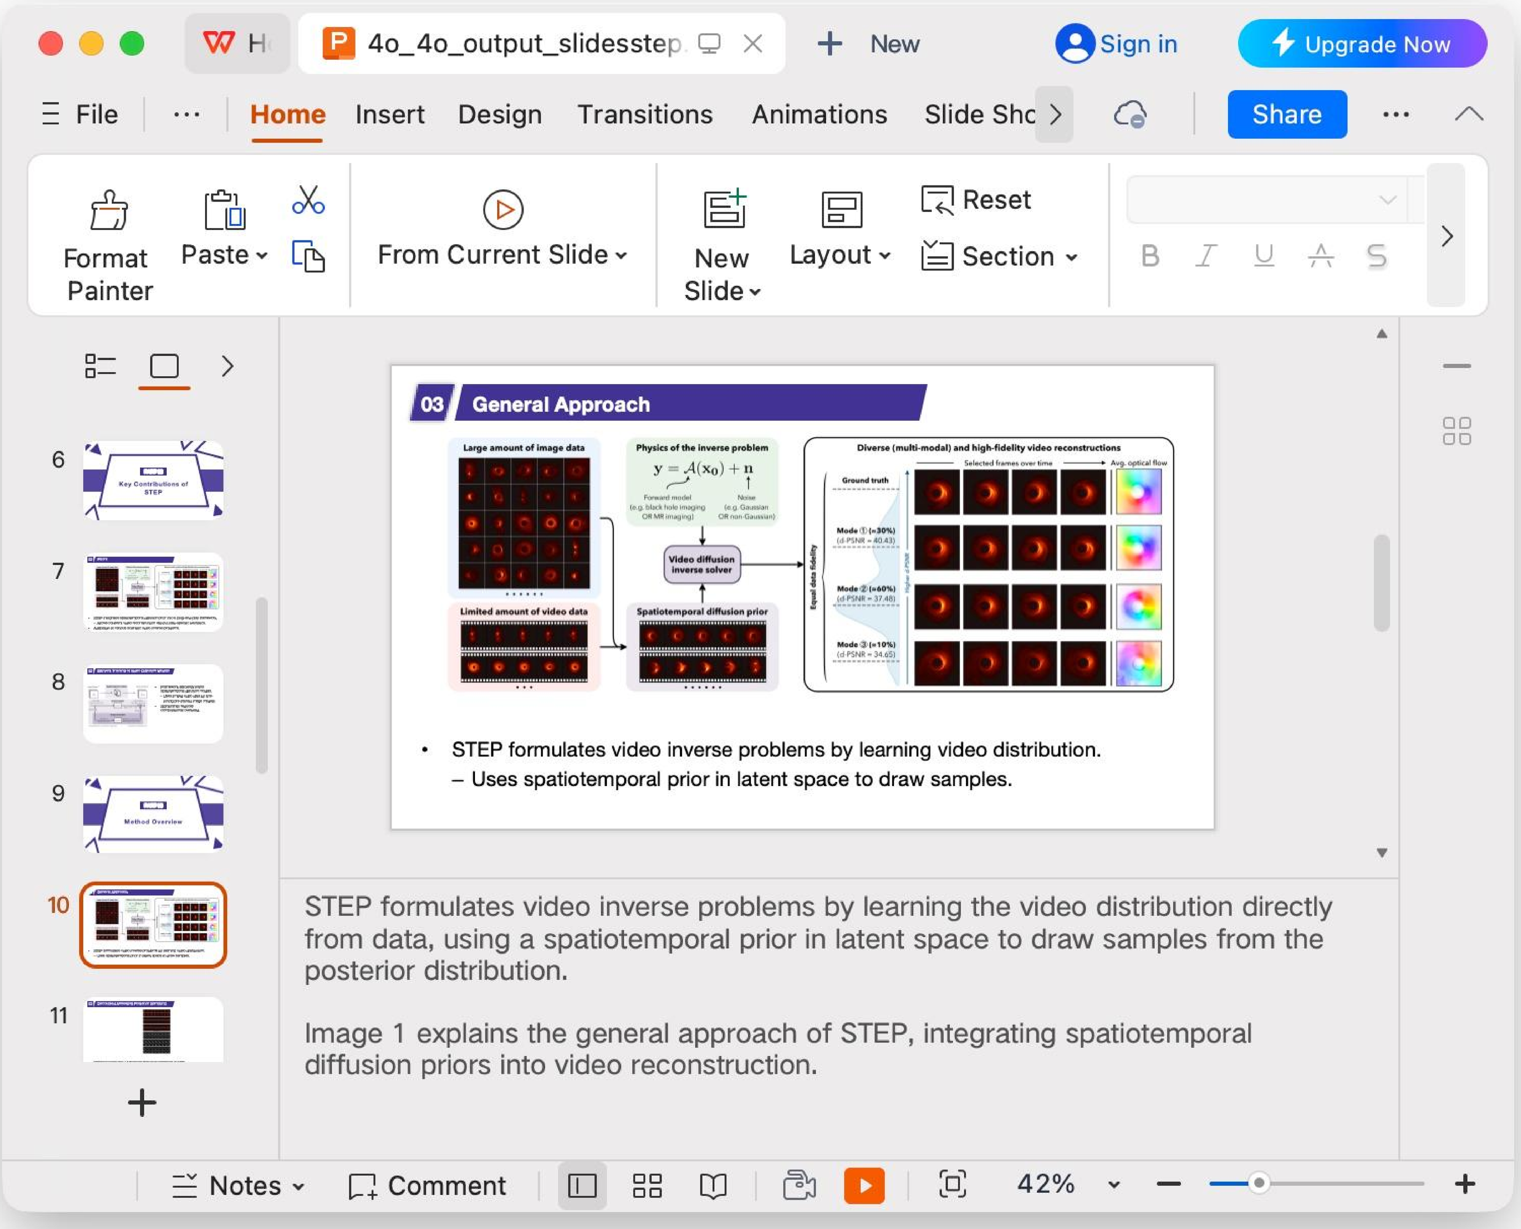
4o_4o_output_slidesstep
03 General Approach
STEP formulates video inverse problems by learning video distribution.
– Uses spatiotemporal prior in latent space to draw samples.
STEP formulates video inverse problems by learning the video distribution directly from data, using a spatiotemporal prior in latent space to draw samples from the posterior distribution.
Image 1 explains the general approach of STEP, integrating spatiotemporal diffusion priors into video reconstruction.

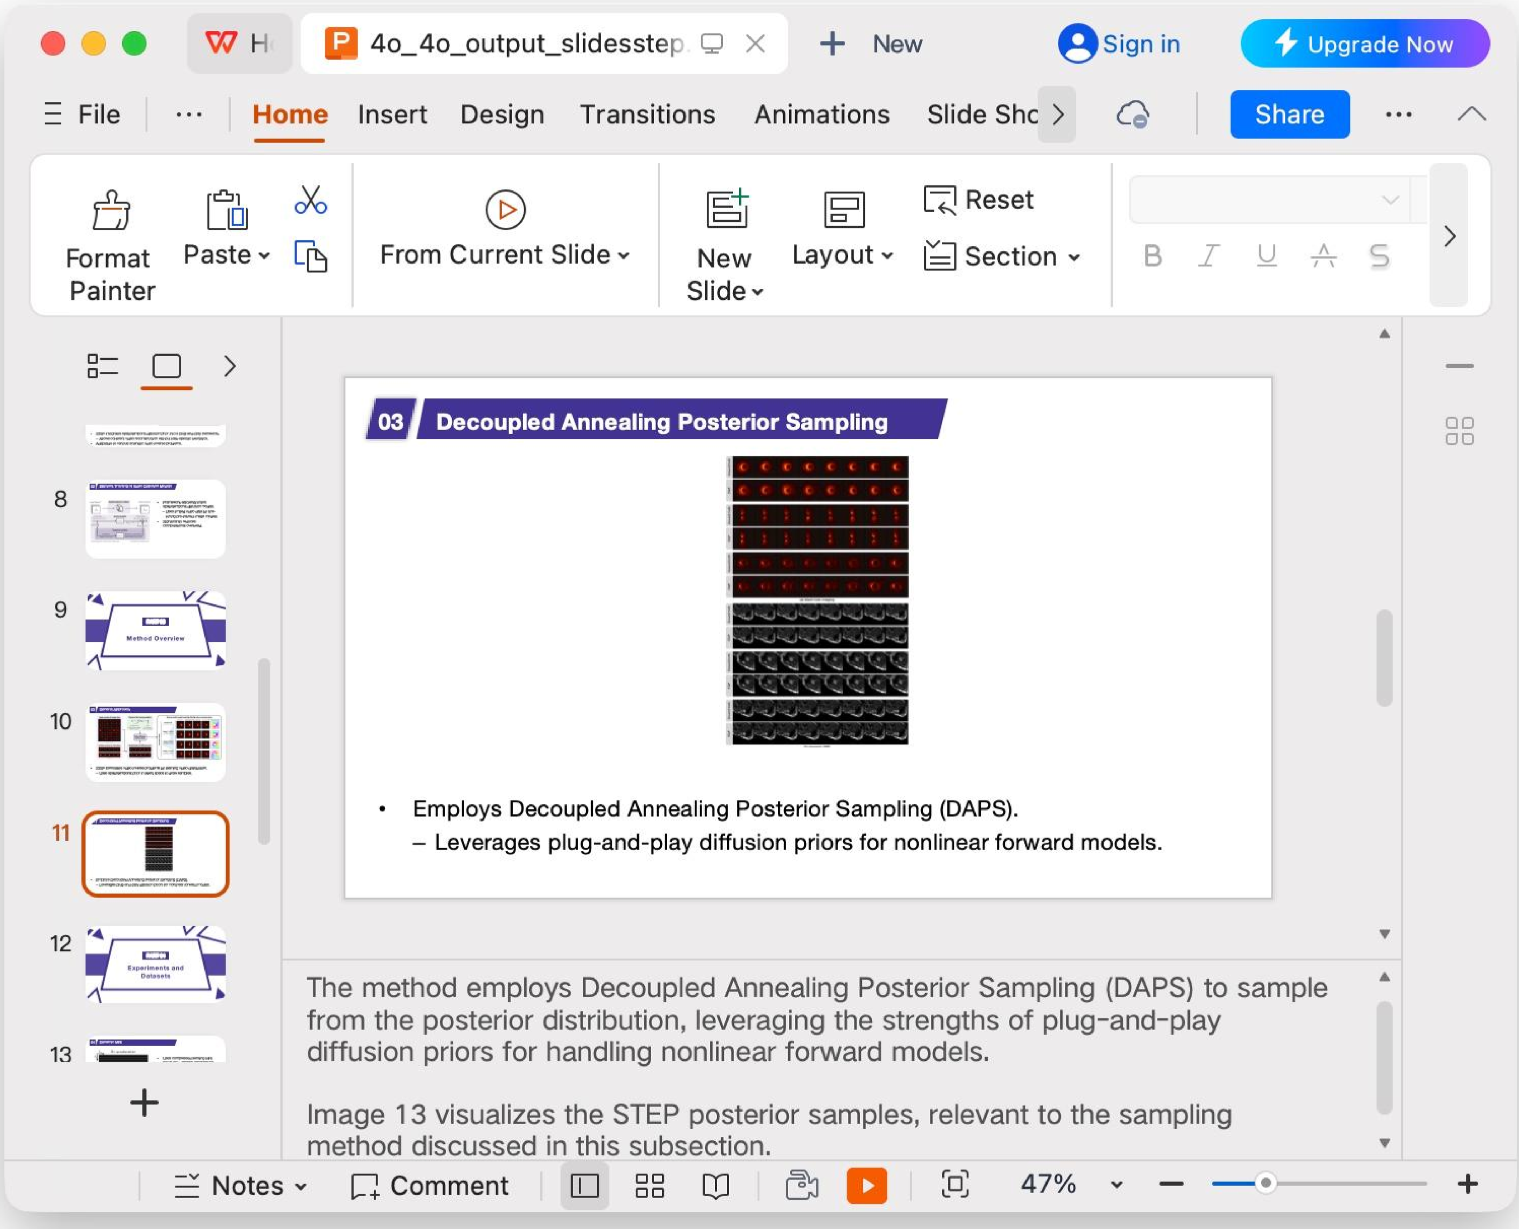
4o_4o_output_slidesstep
03 Decoupled Annealing Posterior Sampling
Employs Decoupled Annealing Posterior Sampling (DAPS).
– Leverages plug-and-play diffusion priors for nonlinear forward models.
The method employs Decoupled Annealing Posterior Sampling (DAPS) to sample from the posterior distribution, leveraging the strengths of plug-and-play diffusion priors for handling nonlinear forward models.
Image 13 visualizes the STEP posterior samples, relevant to the sampling method discussed in this subsection.

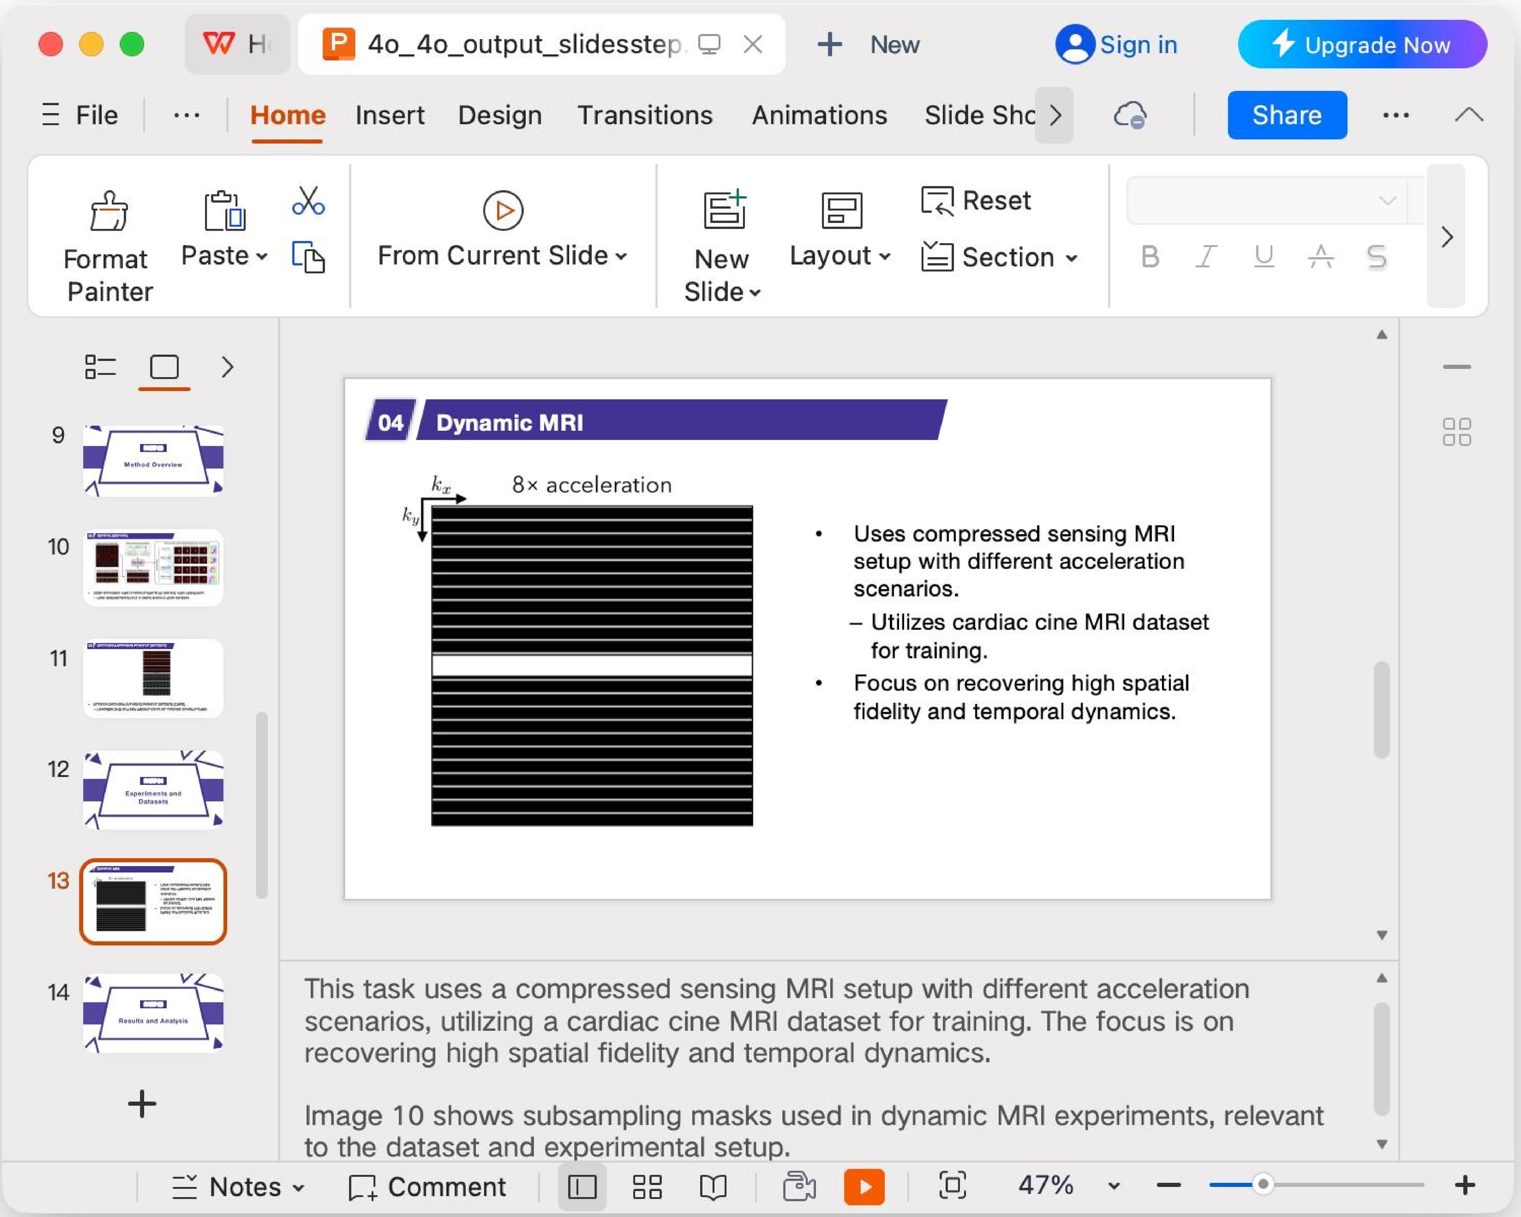
4o_4o_output_slidesstep
04 Dynamic MRI
8× acceleration
Uses compressed sensing MRI setup with different acceleration scenarios.
– Utilizes cardiac cine MRI dataset for training.
Focus on recovering high spatial fidelity and temporal dynamics.
This task uses a compressed sensing MRI setup with different acceleration scenarios, utilizing a cardiac cine MRI dataset for training. The focus is on recovering high spatial fidelity and temporal dynamics.
Image 10 shows subsampling masks used in dynamic MRI experiments, relevant to the dataset and experimental setup.

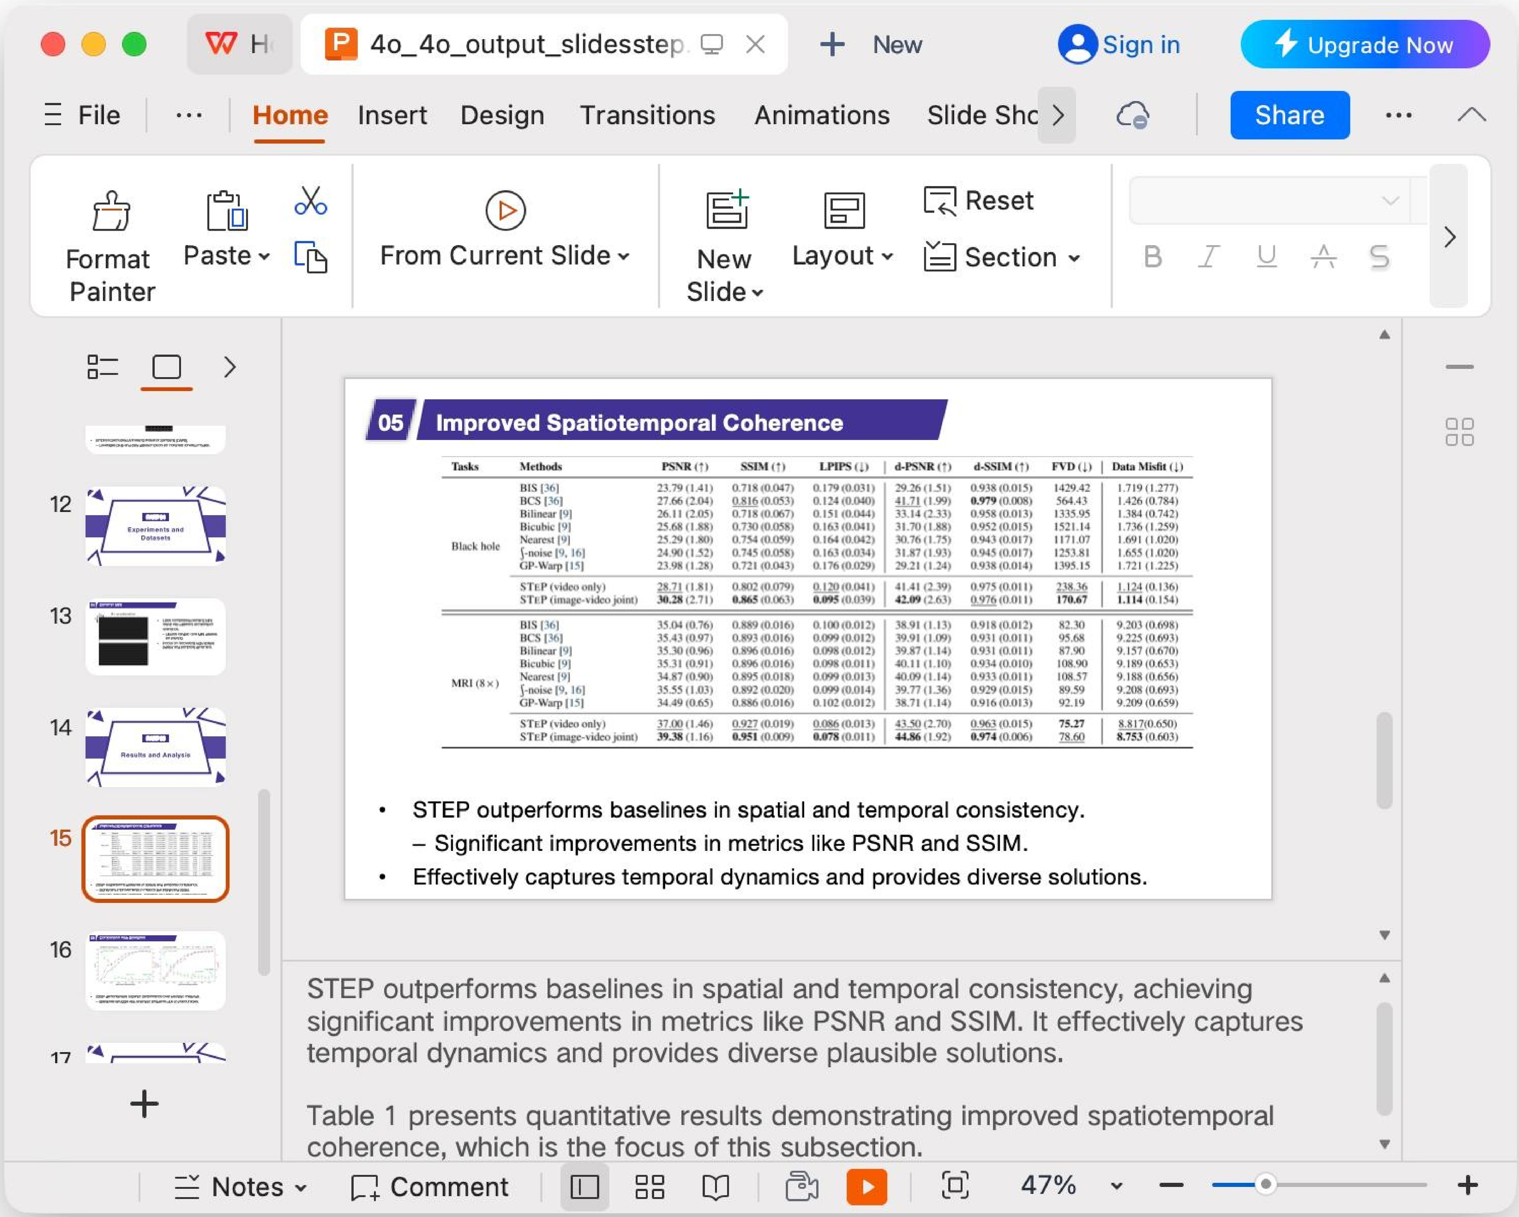
4o_4o_output_slidesstep
05 Improved Spatiotemporal Coherence
STEP outperforms baselines in spatial and temporal consistency.
– Significant improvements in metrics like PSNR and SSIM.
Effectively captures temporal dynamics and provides diverse solutions.
STEP outperforms baselines in spatial and temporal consistency, achieving significant improvements in metrics like PSNR and SSIM. It effectively captures temporal dynamics and provides diverse plausible solutions.
Table 1 presents quantitative results demonstrating improved spatiotemporal coherence, which is the focus of this subsection.

Home | 4o_4o_output_slidesstep | New | Upgrade Now

File | Home | Insert | Design | Transitions | Animations | Slide Show | Review | Share

Format Painter | Paste | From Current Slide | New Slide | Layout | Reset | Section

## 02 Introduction of Spatiotemporal Diffusion Prior

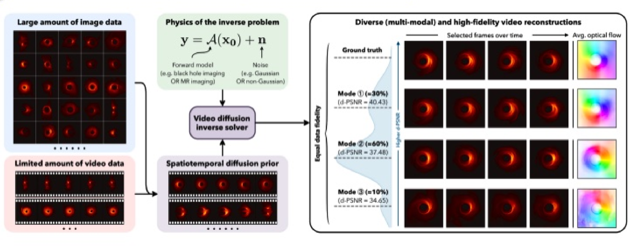


- STEP integrates spatiotemporal diffusion prior into a plug-and-play framework.
  – Allows coherent video reconstruction without task-specific heuristics.
- Adaptable to various scientific video inverse problems.

STEP integrates a spatiotemporal diffusion prior into a plug-and-play framework, allowing for coherent video reconstruction without task-specific temporal heuristics. This approach is adaptable to various scientific video inverse problems.

Image 1 provides an overview of the STEP framework, which is central to the introduction of spatiotemporal diffusion priors.

Slide 7 ... | Notes | Comment | 42%
