# Supplementary material for: SlideGen: Collaborative Multimodal Agents for Scientific Slide Generation
Source: arXiv:2512.04529 source file (2026-08-22)
Supplement: Supplementary file 5 [file prompts.pdf]

Layout Agent

system_prompt:
You are SlidePlanBuilder.
Your ONLY task: return a single valid JSON object matching EXACTLY the schema below.
Do NOT include explanations, summaries, markdown code fences, or natural language.

template:
Instructions:
The PowerPoint canvas is **fixed at 13.3 in* 7.5 in** (16:9).You receive five JSON blobs:
1. **raw_result.json** - hierarchical summary of the paper. Structure:
2. **figures.json** - list of sections → subsections → visual assets. Example (keys may vary by paper):
*Each `imageN` or `tableN` value is an index that maps to an image/table file name (`image_2.png`, `table_1.png`, etc.).*
3. **formula_index.json** - flat list of formula images:
4. **image_dims.json** - pixel dimensions for every `image_.png`
5. **table_dims.json** - pixel dimensions for every `table_.png`

What you must do for **every subsection**

1. **Pick the best slide template** from this library and output its `template_id`:

| ID | When to use |
|----|-------------|
| T1_TextOnly | No images/tables |
| T2_ImageRight | 1 image + ≤4 bullets |
| T3_ImageLeft | Mirror of T2 (alternate left/right across consecutive slides) |
| T4_ImageTop | 1 wide image (aspect > 1.6) or table |
| T5_TwoImages | Exactly 2 side-by-side images, no text |
| T5_TwoImages2 | Two side-by-side images on top, with a text block below |
| T7_2x2_TopImage | 2*2 layout: top two blocks are images, bottom two are text |
| T8_2x2_BottomImage | 2*2 layout: top two blocks are text, bottom two are images |
| T9_2x2_AltTextImg | 2*2 layout: images on top-left & bottom-right, text on top-right & bottom-left |
| T10_4Img_2x2Grid | Four images arranged in a 2*2 grid, no text |
| T11_3Img_TopTextBottom | Vertically divided: 3 images on top, text block below |
| T12_3Img_BottomTextTop | Text block on top, 3 square images in one row below |
| T13_3Img | Title on top, followed by 3 evenly spaced images |
| T14_ImageRight_1Formula | Right column has two slots: top-right = one image or one table, bottom-right = one formula; left column = text bullets. Use when the slide has one key equation plus one main visual. |
| T15_ImageLeft_1Formula | Left column has two slots: top-left = one image or one table, bottom-left = one formula; right column = text bullets. Use when the slide has one key equation plus one main visual. |

| T16_1Img_2formula_TopTextBottom | Bottom = text block; top are three rows: row1 = one

image or one table, row2 = one formula, row3 = one formula. Use for one main visual plus two formulas. |
| T17_2Img_1formula_TopTextBottom | Top row: two visuals side by side (each is one image or one table); middle row: one formula; bottom: text block. |
| T18_2formula_TopTextBottom | Top 2 rows: two formulas; bottom: text block. |

2. **Generate hierarchical bullets** summarising the subsection:
   • Up to **6 top-level bullets**.
   • Each top bullet may have **0-6 sub-bullets** (2-level outline).
   • Top bullets ≤ 20 words; sub-bullets ≤ 25 words.

3. **Select visuals** that best support the bullets:
   • **Formulas** belonging to the same subsection should stay **on the same slide whenever possible**; if more than 2, prefer `T11_3Img_TopTextBottom`.
   • **Do not crop or distort images** - preserve original aspect ratio (minor scaling to fit is fine).

4. **Return a single valid JSON object** with the exact schema below - do **NOT** wrap it in markdown.

```json


{
    "slides": [
      {
        "section": "<string>",
        "subsection": "<string>",
        "template_id": "T?_",
        "bullets": [
          {
            "text": "<string>",
            "sub": ["<string>", ...]
          }, ...
        ],
        "images": ["<filename>", ...],
        "tables": ["<filename>", ...],
        "formulas": ["<filename>", ...]
      }, ...
    ]
  }
```

*Use the template-selection rules strictly so that downstream code can rely on them.*
Answer **only** with the JSON.

## You **must** consider each visual's size and aspect ratio

*For every image / table, compute aspect = width ÷ height.*
*Choose the slide template and left/right/top placement based on aspect and* absolute size:
- **Wide** (aspect ≥ 1.6) → best placed across the top (template **T4_ImageTop**), including wide tables.
- **Tall / square** (aspect ≤ 1.0) → best placed on the left or right (templates **T2_ImageRight** or **T3_ImageLeft**).
- If a visual's width is nearly the full slide width, prefer **T4_ImageTop** to avoid excessive down-scaling.

***Never*** *stretch or crop; only scale proportionally to fit placeholders.*

When designing slide layouts, you must carefully consider visual density and legibility constraints—especially for images that are wide or contain fine-grained details.

Such images often become unreadable when downscaled to fit dual-visual layouts like T2_ImageRight, T3_ImageLeft, or T5_TwoImages2.

If multiple visuals(such as two images both with an aspect ratio greater than 1.6) are assigned to the same subsection but combining them would result in overcrowding or poor legibility, first check whether one of them fits better semantically in a neighboring subsection (e.g., covering a related topic or dataset). If so, move it to that subsection and assign a layout that presents it alone.

raw_result:
{{ raw_result_json }}
figures:
{{ figures_json }}
formulas:
{{ formulas_json }}
image_informations:
{{ image_informations_json }}
table_informations:
{{ table_informations_json }}

jinja_args:
- raw_result_json
- figures_json
- formulas_json
- image_informations_json
- table_informations_json

**formula_match**

```
system_prompt: |
  You are an expert assistant tasked with assigning formulas to the most relevant paper sections.
  You will be given:
    1. JSON content of the paper structure, including sections and subsections (with title and description).
    2. A list of formulas with LaTeX, page_no, and the surrounding text context.
  GOAL:
    • Each formula should be assigned to its corresponding subsection, and a subsection may contain multiple formulas.
    • Produce a new JSON object that mirrors the structure of the provided paper_outline_json (sections → subsections).
    • For each subsection, assign zero, one, or multiple formulas.

    • For each assigned formula, include:
       - "formulaN": <formula_id>
       - "reasonN": <reason string> explaining why it's assigned
    • For each formula assigned to a subsection, generate a reason string ("reasonN") that not only explains why the formula is assigned to this specific subsection,
      but also briefly interprets the formula's mathematical meaning or role within the paper.
    • A formula may be assigned to multiple subsections (if conceptually appropriate), but not multiple times in the same subsection.
    • Keys must use correct suffixing: formula, formula1, formula2,... and reason, reason1, reason2,...
    • Keep section/subsection titles exactly as-is. Do not include their full content in the output.
    • The final result should be a single valid JSON structure.
  THINKING STRATEGY:
    • Use the surrounding context and page_no from the formula list to guide assignment.
    • Match concepts using keywords, notation, or nearby words (e.g., if the section talks about "posterior", and the formula mentions p(x|y), that's a match).
    • Try to ensure each early-indexed formula (e.g. formula 1-5) is assigned at least once.
    • Do not assign arbitrarily.

  OUTPUT FORMAT:
  {
    "sections": [
      {
        "title": "<Section Title>",
        "subsections": [
          {
            "title": "<Subsection Title>",
            "formula1": <id>,
            "reason1": "<explanation>",
            "formula2": <id>,
            "reason2": "<explanation>"
          },
          ...
        ]
      },
      ...
    ]
```

```
  }
  CAUTION:
    - Output must be valid JSON only (no comments or explanations).
    - Only include sections/subsections where at least one formula is assigned.
    - Match titles exactly from the original input.
template: |
  Instructions:
    1. Analyze the paper outline: {{ json_content }}
    2. Analyze the list of formulas with their latex and context: {{ formula_information }}
    3. For each subsection, decide which formulas (if any) are conceptually relevant based on content
and wording.
    4. Match carefully using terms, equations, symbols, and latent meaning.
    5. Output a single JSON object following the system_prompt rules.
jinja_args:
  - json_content
  - formula_information
```

layout_agent_fomula_mode1

You are **SlidePlanBuilder**, an expert assistant that converts section/subsection text plus visual-assets metadata into a slide-planning JSON object.
The PowerPoint canvas is **fixed at 13.3 in * 7.5 in** (16:9).
You receive **five** JSON blobs:

1. **raw_result.json** - hierarchical summary of the paper. Structure:

2. **figures.json** - list of sections → subsections → visual assets. Example (keys may vary by paper):
*Each `imageN` or `tableN` value is an index that maps to an image/table file name (`image_2.png`, `table_1.png`, etc.).*

3. **formula_index.json** - flat list of formula images:
4. **image_dims.json** - pixel dimensions for every `image_*.png`
5. **table_dims.json** - pixel dimensions for every `table_*.png`

---
## What you must do for **every subsection**

1. **Pick the best slide template** from this library and output its `template_id`:

| ID | When to use |
|----|-------------|
| T1_TextOnly | No images/tables |
| T2_ImageRight | 1 image + ≤4 bullets |
| T3_ImageLeft | Mirror of T2 (alternate left/right across consecutive slides) |
| T4_ImageTop | 1 wide image (aspect > 1.6) |
| T5_TwoImages | Exactly 2 side-by-side images, no text |
| T5_TwoImages2 | Two side-by-side images on top, with a text block below |
| T7_2x2_TopImage | 2*2 layout: top two blocks are images, bottom two are text |
| T8_2x2_BottomImage | 2*2 layout: top two blocks are text, bottom two are images |
| T9_2x2_AltTextImg | 2*2 layout: images on top-left & bottom-right, text on top-right & bottom-left |
| T10_4Img_2x2Grid | Four images arranged in a 2*2 grid, no text |
| T11_3Img_TopTextBottom | Vertically divided: 3 images on top, text block below |
| T12_3Img_BottomTextTop | Text block on top, 3 square images in one row below |
| T13_3Img | Title on top, followed by 3 evenly spaced images |

2. **Generate hierarchical bullets** summarising the subsection:
   • Up to **4 top-level bullets**.
   • Each top bullet may have **0-3 sub-bullets** (2-level outline).
   • Top bullets ≤ 20 words; sub-bullets ≤ 15 words.

3. **Select visuals** that best support the bullets:
   • Max 2 images/tables **and** max 2 formulas per slide.
   • **Formulas** belonging to the same subsection should stay **on the same slide whenever**

**possible**; if more than 2, prefer `T11_3Img_TopTextBottom`.

- **Do not crop or distort images** - preserve original aspect ratio (minor scaling to fit is fine).

4. **Return a single valid JSON object** with the exact schema below - do **NOT** wrap it in markdown.

```json
{
 "slides": [
  {
   "section": "<string>",
   "subsection": "<string>",
   "template_id": "T?_*",
   "bullets": [
    {
     "text": "<string>",
     "sub": ["<string>", ...]
    }, ...
   ],
   "images": ["<filename>", ...],
   "tables": ["<filename>", ...],
   "formulas": ["<filename>", ...]
  }, ...
 ]
}
```

*Use the template-selection rules strictly so that downstream code can rely on them.*
Answer **only** with the JSON.

## You **must** consider each visual's size and aspect ratio

* For every image / table, compute **aspect = width ÷ height**.
* Choose the slide template and left/right/top placement based on **aspec**t *and* absolute size:
  - **Wide** (aspect ≥ 1.6) → best placed across the top (template **T4_ImageTop**).
  - **Tall / square** (aspect ≤ 1.0) → best placed on the left or right (templates **T2_ImageRight** or **T3_ImageLeft**).
  - If a visual's width is nearly the full slide width (≈ 12 in or more in pixel equivalent), prefer **T4_ImageTop** to avoid excessive down-scaling.
* **Never** stretch or crop; only scale proportionally to fit placeholders.

```
template: |
 raw_result:
 ```{{ raw_result_json }}```
 figures:
 ```{{ figures_json }}```
 formulas:
 ```{{ formulas_json }}```
 image_informations:
```
```

````
```{{ image_informations_json }}```
 table_informations:
 ```{{ table_informations_json }}```


jinja_args:
 - raw_result_json
 - figures_json
 - formulas_json
````

## figure_match

system_prompt: |
You are an expert assistant tasked with assigning images and tables to the most relevant paper sections.
You will be given:
1. JSON content of the paper outline, including each section's title and a brief description.
2. A list of images (image_information) with captions and size constraints.
3. A list of tables (table_information) with captions and size constraints.

GOAL
• Produce a JSON object that mirrors the hierarchy of paper_outline_json (sections → subsections).
• For each subsection, assign zero, one, or multiple items from image_information and/or table_information.
• Keys inside a subsection must follow:
- image1, image2, … with matching reason / reason1, …
- table1, table2, … with matching reasonT1, reasonT2, …
• The same image or table **may** appear in multiple subsections.
• Ensure that image IDs 1 to 5 are each assigned to at least one subsection if a reasonable conceptual match exists.
• If multiple images or tables match a section well, include all of them. Assign each item only once per section, using different keys: e.g., "image", "image1", "table", "table1", etc.
• If assigning an image, specify “image”: <id>, where <id> is the identifier of the chosen image from “image_information”.
• If assigning a table, specify “table”: <id>, where <id> is the identifier of the chosen table from “table_information”.
• Include an additional “reason”, "reason1", etc. field briefly explaining why this assignment was made (e.g., how the image/table relates to the section content).
• If no image or table is assigned to a given section, omit that section from the final JSON (i.e., only list sections where you actually assign something).
• Keep all section / subsection titles exactly as in the input; omit their “content”.

IMPORTANT:
• The assignment should not be arbitrary. It must be logically consistent with the section’s description and the provided caption for the image or table.
• Do not produce any layout properties or subsections here.
• The final output must be a single JSON object, mapping from section names to the chosen image/table ID plus the “reason” field.
• Extra note: If multiple images or tables are suitable, select the single best one and assign only that.
• If “image_information” or “table_information” is empty, you may end up assigning nothing to any section.

template: |
Instructions:
1. Read and analyze the paper's sections from {{ json_content }} .
2. Look at {{ image_information }} and {{ table_information }}. Determine content-fit:
- If a section's description or subject matter matches well with a given image/table caption, consider assigning it.
- If multiple images or tables seem relevant, choose the single best fit.

- If none of the images or tables are relevant, or if none are provided, do not assign anything for that section.

3. Produce a single JSON object. Each key is the exact name of a top-level section (e.g., "Introduction", "Methods", "Results"), and the value is an object with:
   - "image": image_id or "table": table_id
   - "reason": short explanation describing why the image/table is assigned
4. If no assignment is made for a section, exclude that section from the JSON.
6. Ensure your final response strictly follows JSON syntax with no extra commentary.
7. Keep the original hierarchy (sections → subsections).
8. Use imageN / reason(N-1) and tableN / reasonTN naming as described.
9. No image/table reuse limits across subsections, but do not repeat an item twice inside the same subsection.

Example output format if two sections are assigned:

```
{
  "sections": [
    {
      "title": "Motivation And Background",
      "subsections": [
        {
          "title": "Challenges in Scientific Video Reconstruction",
          "image1": 1,
          "reason": "Image 1 illustrates sparse sampling and spatiotemporal gaps discussed in this subsection.",
          "image2": 2,
          "reason1": "Image 2 compares reconstruction quality across sampling densities, matching the narrative."
        },
        {
          "title": "Limitations of Current Diffusion Models",
          "image1": 3,
          "reason": "Image 3 visualizes frame-wise temporal incoherence produced by existing diffusion models."
        }
      ]
    },
    {
      "title": "Related Work And Limitations",
      "subsections": [
        {
          "title": "Existing Video Inverse Problem Approaches",
          "table1": 1,
          "reasonT1": "Table 1 lists prior methods and evaluation metrics referenced in this subsection.",
          "image1": 4,
          "reason": "Image 4 shows qualitative outputs of baseline approaches highlighted here."
        },
        {
          "title": "Plug-and-Play Diffusion Priors",
          "image1": 5,
```

```
  "reason": "Image 5 presents an overview diagram of the PnPDP framework emphasized in this
subsection."
          }
        ]
      }
    ]
  }

jinja_args:
  - json_content
  - image_information
  - table_information
```

**generate_question_detail**

```
system_prompt: |
  You are a Question-Generation agent for academic slides.
  Your task is to read the supplied Markdown text (``document_markdown``) and
  produce exactly 50 multiple-choice QA items whose answers can be located
  verbatim or almost verbatim in that text.
  The questions must be suitable for conference-slide-deck readers: avoid deep
  theoretical proofs, reference lists, or citation minutiae.
  Follow all guidelines below precisely.

template: |
  ====================================================================
  INSTRUCTIONS
  ====================================================================
  1. Carefully read the Markdown in ``document_markdown``.
  2. Write 50 factual, answerable-from-text questions.
     • Each question must map to one clear sentence/phrase in the slide-deck text.
     • No duplicate or near-duplicate wording.
     • Vary difficulty from easy "headline" facts to specific numeric or
       procedural details.
  3. Distribute the 50 questions across the following slide-deck-friendly aspects.
     Aim for at least 2-5 questions per aspect, and ensure every aspect
     appears at least once.
       A. Title & authorship (title, author names, affiliations, keywords)
       B. Motivation / problem statement / research gap
       C. Objectives or hypotheses
       D. Dataset(s) or experimental materials
       E. Methodology (algorithms, model architecture, workflow steps)
       F. Key parameters or hyper-parameters (values, settings)
       G. Evaluation metrics or criteria
       H. Quantitative results (numbers in tables, charts)
       I. Qualitative findings, figures, or illustrative examples
       J. Comparative or ablation study results
       K. Conclusions, implications, or contributions
       L. Limitations or future work
       M. Definitions of domain-specific terms or abbreviations
  4. EXCLUDE references, citations, author acknowledgements, and any text
     that would not appear on a standard slide-deck.
  5. Use the following JSON-for-each format (exact spelling & casing):
     {
       "Question X": {
         "aspect": "<A-M>",          <-- single letter from list above
         "question": "<single sentence>",
         "options": [
           "A. <choice 1>",
           "B. <choice 2>",
           "C. <choice 3>",
           "D. <choice 4>"
         ],
         "answer": "<Letter>. <exact correct option text>"
```

```
  },
     ...
   }
   Formatting rules
     • Include the "aspect" key to show coverage; no other keys allowed.
     • Exactly four options labelled A-D.
     • Put the correct option text verbatim in the "answer" field, preceded
       by its letter.
     • Distractors must be plausible, the same type/scale as the correct
       answer, and not lifted verbatim from other parts of the text.
6. Output only the final JSON object containing 50 items—nothing else.
7. The number of correct answers for each choice should be approximately
   balanced across A-D.

----------------------------------------------------------------
document_markdown:
{{ document_markdown }}
----------------------------------------------------------------

 Return ONLY the JSON with 50 questions below

jinja_args:
 - document_markdown
```

**generate_question_understanding**

system_prompt: |
You are a Question-Generation agent.
Your task is to read the supplied Markdown text (``document_markdown``) and create **exactly 50 multiple-choice questions** that capture a *high-level understanding* of the work—its purpose, novelty, core approach, and overall findings.
Every question must still be answerable by locating explicit sentences or phrases in the text; do not require inference that is absent from the slide-style content.

template: |

==========================================================================

INSTRUCTIONS

==========================================================================

1. Read the Markdown in ``document_markdown`` closely.
2. Draft 50 factual questions that probe the reader's global grasp of the paper (e.g., "What problem does the study address?").
   • Avoid low-level numeric settings, code snippets, or reference lists.
   • Vary wording and avoid duplicates.
3. Cover all of the following *high-level* aspects—each must appear at least twice to guarantee breadth:
   A. Research domain & background context
   B. Central problem / motivation / research gap
   C. Primary goal, hypothesis, or research question
   D. Key contributions or novelty statements
   E. Overall methodology or workflow (summarized)
   F. Principal findings or headline quantitative results
   G. Qualitative insights or illustrative examples
   H. Implications, applications, or significance
   I. Limitations or future-work directions
   J. Main conclusions or take-home messages
4. EXCLUDE citations, granular hyper-parameters, precise numeric tables, and acknowledgements—stick to slide-level overview content.
5. Return the questions in the following *strict* JSON schema:

```
{
 "Question X": {
   "aspect": "<A-J>",          <-- single capital letter above
   "question": "<one concise sentence>",
   "options": [
     "A. <choice 1>",
     "B. <choice 2>",
     "C. <choice 3>",
     "D. <choice 4>"
   ],
   "answer": "<Letter>. <exact correct option text>"
 },
 ...
}
```

Formatting rules

- Exactly four labelled options (A-D); one is correct.
  - The "answer" field must contain the correct option's letter, a period, and the *exact* option text.
  - Distractors must be plausible, topically related, and not verbatim copies of unrelated sentences.

6. Produce **only** the final JSON object with 50 entries—no commentary, headers, or extra lines.
7. The number of correct answers for each choice should be approximately balanced across A-D.

---------------------------------------------------------------

document_markdown:
{{ document_markdown }}

---------------------------------------------------------------

Output ONLY the JSON with 50 questions below

jinja_args:
- document_markdown

## ppteval_coherence

You are an unbiased presentation analysis judge responsible for evaluating the coherence of the presentation. Please carefully review the provided summary of the presentation, assessing its logical flow and contextual information. Each score level requires that all evaluation criteria meet the standards of that level.
Scoring Criteria (Five-Point Scale)

1 Point:
The logical structure is chaotic, making it difficult for the audience to understand.

2 Points:
The logical structure is generally reasonable, with minor issues in transitions.

3 Points:
The presentation demonstrates a clear and logical structure, with smooth transitions between sections. However, it lacks essential background information.

4 Points:
The presentation features a well-organized logical flow and includes basic background information (e.g., speaker, date, or institution).

5 Points:
The narrative structure is engaging and meticulously organized with detailed and comprehensive background information(speaker/institution, date, and acknowledgments/conclusion) included.

Example Output:

```
{
  "reason": "xx",
  "score": int
}
```

Input:
{{presentation}}

Let's think step by step and provide your judgment, focusing exclusively on the dimensions outlined above and strictly follow the criteria.

ppteval_style

You are an unbiased presentation analysis judge responsible for evaluating the visual appeal of slides. Please carefully review the provided description of the slide, assessing their aesthetics only, and provide your judgment in a JSON object containing the reason and score. Each score level requires that all evaluation criteria meet the standards of that level.

Scoring Criteria (Five-point scale):

1 Point (Poor):
There is a conflict between slide styles, making the content difficult to read.

2 Points (Fair):
The slide uses monotonous colors(black and white), ensuring readability while lacking visual appeal.

3 Points (Average):
The slide employs a basic color scheme; however, it lacks supplementary visual elements such as icons, backgrounds, images, or geometric shapes(like rectangles), making it look plain.

4 Points (Good):
The slide uses a harmonious color scheme and contains some visual elements(like icons, backgrounds, images, or geometric shapes); however, minor flaws may exist in the overall design.

5 Points (Excellent):
The style of the slide is harmonious and engaging, the use of supplementary visual elements like images and geometric shapes enhances the slide's overall visual appeal.

Example Output:

```
{
  "reason": "xx",
  "score": int
}
```

Input: {{descr}}
Please evaluate the slide step by step, ensuring your judgment strictly adheres to the scoring criteria.

Outline JSON

{
"**metadata**": {
"title": "A Touch, Vision, and Language Dataset for Multimodal Alignment",
"author": "Letian Fu; Gaurav Datta; Huang Huang; William Chung-Ho Panitch; Jaimyn Drake; Joseph Ortiz; Mustafa Mukadam; Mike Lambeta; Roberto Calandra; Ken Goldberg",
"publish date": "2024",
"organization": "UC Berkeley; Meta AI; TU Dresden"
},
"**sections**": [
{
"title": "Motivation: Why Integrate Touch With Vision And Language?",
"**subsections**": [
{
"title": "Gaps In Multimodal Models",
"content": "Most multimodal generative and alignment models focus on visual, textual, and sometimes audio or action signals, leaving tactile sensing underexplored. Yet touch captures material, texture, compliance, and force-related semantics vital for manipulation and human-like perception. A lack of open-vocabulary tactile-language data and difficulty synchronizing tactile with visual context impede progress. This work addresses scarce labels, subjective descriptions, and misalignment by proposing a dataset and models that align tactile, visual, and linguistic representations."
},
{
"title": "Why Does This Matter?",
"content": "Combining touch with vision and language can yield agents that more robustly infer material properties and contact states, improving open-vocabulary understanding and manipulation. The approach promises better generalization than vision-only models, enabling text-grounded tactile understanding and generation. It may benefit robotics, haptics research, and broader multimodal AI by providing a scalable path to tactile-language supervision via pseudo-labels."
}
]
},
{
"title": "Related Work And Limitations Of Existing Approaches",
"**subsections**": [
{
"title": "Multimodal Encoders And Alignment",
"content": "CLIP and derivatives align vision and language using contrastive learning; ImageBind extends to more modalities but primarily binds them through vision. Other works include masked multimodal pretraining and parameter-efficient alignment with LLMs. However, direct tactile-language alignment is typically absent, and tactile is often only bound to vision, limiting tactile semantic coverage."
},
{
"title": "Tactile Perception And Datasets",
"content": "Prior tactile-vision efforts address closed-set material or cloth classification and manipulation, often in lab settings, with limited vocabulary and diversity. Some datasets integrate audio or point clouds, but open-vocabulary tactile-language labels are missing. Concurrent efforts bind touch to vision without finetuning LLMs, leaving room for stronger tactile-language alignment

Outline JSON


```
and generation."
            },
            {
                "title": "Training From Pseudo-Labels",
                "content": "Self-training and pseudo-labeling reduce annotation costs. Recent LLM/VLM pipelines use GPT-generated instruction data, but typically with matching input-output modalities. Here, vision-only GPT-4V generates tactile descriptions from images to supervise alignment with tactile data, expanding labeled coverage while acknowledging potential label noise."
            }
        ]
    },
    {
        "title": "Key Contributions Of This Work",
        "subsections": [
            {
                "title": "TVL Dataset: 44K Vision\u2013Tactile\u2013Language Triplets",
                "content": "A new dataset with 43,741 in-contact vision\u2013tactile pairs and open-vocabulary labels: 10% human-annotated (SSVTP) and 90% GPT-4V pseudo-labeled (HCT). The dataset spans in-the-wild settings, synchronized acquisition, and 254 unique tactile adjectives. A 99%/1% split is used with a human-labeled test set."
            },
            {
                "title": "Vision- And Language-Aligned Tactile Encoder",
                "content": "A tactile encoder trained via pairwise contrastive learning across tactile\u2013language, tactile\u2013vision, and vision\u2013language pairs, aligning tactile inputs directly to CLIP\u2019s latent space. Training strategies include inclusion of background (no-contact) frames labeled as \u2018background,\u2019 projector removal for vision/text, and randomized adjective subsets to improve robustness."
            },
            {
                "title": "TVL-LLaMA: Touch\u2013Vision\u2013Language Generation",
                "content": "A multimodal generation model finetuning LLaMA2-7B with TVL encoders to produce tactile descriptions from tactile and visual inputs. Two-stage training follows ImageBind-LLM style fusion, with additional instruction data (LLaVA CC3M, Alpaca, LLaVA 150K) to counter safety refusals and improve instruction-following."
            }
        ]
    },
    {
        "title": "Dataset: Collection, Cleaning, And Language Labeling",
        "subsections": [
            {
                "title": "Hardware And Synchronous Data Collection",
                "content": "A 3D-printed handheld rig integrates a DIGIT tactile sensor and a Logitech BRIO webcam to capture synchronized tactile and visual streams at 30 Hz during approach, contact, slide, and withdrawal trajectories. Five human collectors gathered 20 hours of diverse in-the-wild interactions ensuring the contact region remains in view, boosting variety and alignment fidelity."
            },
            {
```

Outline JSON


```
            {
               "title": "Cleaning: Contact Versus No-Contact Frames",
               "content": "Using a pretrained tactile encoder, frames are categorized by cosine similarity to a background embedding; contact is flagged when similarity drops below 0.6. The final dataset includes 43,741 in-contact and 169,292 out-of-contact pairs. Contact frames are used primarily for training alignment and evaluation; a portion of no-contact frames aids generalization."
            },
            {
               "title": "Language Labeling: Human And GPT-4V Pseudo-Labels",
               "content": "SSVTP pairs are human-labeled using up to five adjectives drawn from a curated 400-word tactile vocabulary. HCT labels are generated by GPT-4V using both full and cropped images around the contact. Failures (e.g., occlusions, blur) are mitigated by labeling nearby frames within a trajectory or dropping unlabeled trajectories. Overall, 39,154 pseudo-labeled images are produced."
            },
            {
               "title": "Dataset Statistics And Split",
               "content": "SSVTP: 4,587 pairs; HCT: 39,154 in-contact and 169,292 no-contact pairs across 1,486 trajectories. A 99/1 train-test split is used; the test set (402 pairs) is human-labeled. GPT-4V averages 4.25 adjectives per item vs. 2.70 for humans, covering 254 distinct descriptors and yielding a long-tailed vocabulary distribution."
            }
         ]
      },
      {
         "title": "Method Overview And Technical Design",
         "subsections": [
            {
               "title": "Contrastive Alignment Across All Modality Pairs",
               "content": "Unlike ImageBind\u2019s vision-centric binding, TVL optimizes InfoNCE across tactile\u2013language, tactile\u2013vision, and vision\u2013language. The tactile encoder (ViT-Tiny/Small/Base) is randomly initialized and projects to CLIP\u2019s latent space; vision/text use frozen OpenCLIP without additional projectors. Training shuffles and subsets language adjectives per sample for label diversity and includes 10% no-contact frames labeled \u2018background\u2019 to curb overfitting."
            },
            {
               "title": "Instruction Tuning With Multimodal Tokens",
               "content": "TVL-LLaMA follows ImageBind-LLM/LLaMA-Adapter fusion, averaging vision and tactile latents into a single token and using a zero-initialized gate and LoRA for efficient alignment. Pretraining uses LLaVA CC3M subset and TVL (empty tactile image for CC3M), followed by finetuning on TVL, Alpaca, and LLaVA 150K to improve instruction following and safety-guarded refusals."
            },
            {
               "title": "Prompting And Preprocessing Choices",
               "content": "Prompts are diversified for tactile description generation during fine-tuning; evaluation uses GPT-4 grading prompts with order randomization to reduce bias.
```

Outline JSON


Tactile preprocessing includes padding, resizing to 224\u00d7224, optional background subtraction, and normalization. Vision preprocessing uses CLIP statistics and tailored crops to keep sensor contact visible, matching GPT-4V labeling conditions."
}
]
},
{
"title": "Experiments, Datasets, And Evaluation Protocols",
"**subsections**": [
{
"title": "Open-Vocabulary Cross-Modal Classification",
"content": "On the human-labeled TVL test set (402-way), top-1/top-5 accuracy is computed for tactile\u2013vision and tactile\u2013language. To handle synonymy and order sensitivity in CLIP text embeddings, a synonym-expanded label set is built via GPT-4; cosine similarity thresholds define correctness. Vision\u2013text uses OpenCLIP scores. Baselines include SSVTP encoders and CLIP."
},
{
"title": "TVL Benchmark For Tactile Description Generation",
"content": "Given full image, cropped image, and tactile frame, models output up to five adjectives. GPT-4 scores responses against human labels from 1\u201310 with rationales. Models compared include GPT-4V, LLaVA variants, ViP-LLaVA, LLaMA-Adapter, BLIP-2, InstructBLIP, SSVTP-LLaMA, and TVL-LLaMA (Tiny/Small/Base). Statistical significance is assessed via paired t-tests."
},
{
"title": "Additional Tasks And Ablations",
"content": "A zero-shot binary object category test (fabric vs. plastic) illustrates downstream utility. Ablations analyze encoder size, disabling tactile\u2013text loss, modality removal, no-contact data mixing, prompt variants, background subtraction, training subsets (SSVTP vs. HCT vs. TVL), and freezing vs. finetuning the LLM. Overfitting to pseudo-labels and distribution shift between human and GPT-4V labels are examined."
}
]
},
{
"title": "Results And Comparative Analysis",
"**subsections**": [
{
"title": "Classification Performance",
"content": "TVL tactile encoders achieve strong tactile\u2013vision (up to 81.7% top-1) and tactile\u2013text (up to 36.7% top-1) accuracy on the TVL test set, outperforming SSVTP on in-the-wild data and surpassing OpenCLIP\u2019s vision\u2013text alignment for tactile semantics. Direct tactile\u2013text supervision is crucial; removing it reduces tactile\u2013text accuracy markedly."
},

Outline JSON

{
"title": "TVL Benchmark: Generation Scores",
"content": "TVL-LLaMA outperforms GPT-4V by at least 12% and open-source VLMs by larger margins, with significant p-values. Improvements hold across SSVTP (lab) and HCT (in-the-wild) subsets, showing benefits from limited human labels and extensive pseudo-labels. SSVTP-LLaMA, lacking tactile\u2013text pretraining, underperforms, underscoring the need for explicit tactile-language alignment."
},
{
"title": "Ablation Insights And Sensitivity",
"content": "Including all modality pair losses boosts alignment; background subtraction and limited no-contact data mitigate overfitting and improve downstream scores. Encoder size trades off robustness and overfitting to pseudo-labels. Prompt format has minor effects. Freezing the LLM can match finetuning in some settings, suggesting strong encoder alignment to language space."
}
]
},
{
"title": "Limitations, Conclusion, And Future Directions",
"**subsections**": [
{
"title": "Current Limitations",
"content": "Vision-derived pseudo-labels may misdescribe tactile sensations when contact is occluded or ambiguous. Distribution shifts between GPT-4V pseudo-labels and human test labels can cause overfitting or evaluation gaps. Safety tuning in LLaMA2 required additional instruction data to avoid refusals. The vocabulary distribution is long-tailed with some noisy descriptors."
},
{
"title": "Conclusion And Broader Impact",
"content": "TVL provides a large-scale, synchronized vision\u2013tactile dataset with open-vocabulary labels, enabling a tactile encoder aligned with both vision and language and a TVL-LLaMA capable of generating tactile descriptions. Results demonstrate improved tactile-vision-language alignment and generation over strong baselines. The work advances embodied AI and robotic manipulation through richer multimodal grounding."
},
{
"title": "Future Work",
"content": "Scale human-labeled coverage, diversify environments and sensors, improve pseudo-label uncertainty handling, and explore richer task formulations (e.g., action-conditioned tactile reasoning). Investigate better fusion strategies beyond latent averaging, domain adaptation for occlusion or lighting, and extended downstream tasks such as open-world material and affordance understanding."
}
]
}
]
}

Mapper JSON for images and tables


```
{
  "sections": [
    {
      "title": "Proposed Method: Multi-Turn Program Synthesis",
      "subsections": [
        {
          "title": "Multi-Turn Approach",
          "image1": 1,
          "reason": "Image 1 provides an illustrative example of the Multi-Turn Programming Benchmark, which aligns with the multi-turn approach described in this subsection."
        },
        {
          "title": "Advantages of Multi-Turn Synthesis",
          "table1": 3,
          "reasonT1": "Table 3 shows evaluation results on the Multi-Turn Programming Benchmark, directly related to the advantages of multi-turn synthesis discussed here."
        }
      ]
    },
    {
      "title": "Experiments and Evaluation",
      "subsections": [
        {
          "title": "Single-Turn Evaluation",
          "table1": 1,
          "reasonT1": "Table 1 presents evaluation results on the HumanEval benchmark, relevant to the single-turn evaluation discussed in this subsection."
        },
        {
          "title": "Multi-Turn Evaluation",
          "image1": 2,
          "reason": "Image 2 shows the difference in pass rates between single-turn and multi-turn formulations, which is pertinent to the multi-turn evaluation."
        }
      ]
    },
    {
      "title": "Results and Analysis",
      "subsections": [
        {
          "title": "Performance on Benchmarks",
          "table1": 4,
          "reasonT1": "Table 4 compares multi-turn and single-turn specifications, which is relevant to the performance analysis on benchmarks."
        }
      ]
    },
```

```
    {
        "title": "Model Training and Datasets",
        "subsections": [
            {
                "title": "Datasets Used",
                "table1": 7,
                "reasonT1": "Table 5 provides statistics for training corpora, which is relevant to the datasets used for training CODEGEN models."
            }
        ]
    }
  ]
}
```

Arranger JSON for images and tables


```
{
  "slides": [
    {
      "section": "Introduction to Prompt Caching",
      "subsection": "Introduction to Prompt Caching",
      "template_id": "T4_ImageTop",
      "bullets": [
        {
          "text": "Prompt caching leads to data-dependent timing variations.",
          "sub": [
            "Cached prompts are processed faster than non-cached ones.",
            "This can result in side-channel timing attacks."
          ]
        },
        {
          "text": "Shared caches across users increase privacy risks.",
          "sub": [
            "If caches are shared, attackers can infer prompt information."
          ]
        }
      ],
      "images": [
        "Auditing_Prompt_Caching_in_Language_Model_APIs-picture-1.png"
      ],
      "tables": [],
      "formulas": []
    },
    {
      "section": "Introduction to Prompt Caching",
      "subsection": "Risks of Timing Attacks",
      "template_id": "T1_TextOnly",
      "bullets": [
        {
          "text": "Timing differences can be exploited by attackers.",
          "sub": [
            "Attackers can infer information about other users' prompts.",
            "Global cache sharing poses significant privacy concerns."
          ]
        }
      ],
      "images": [],
      "tables": [],
      "formulas": []
    },
    {
      "section": "Preliminaries and Assumptions",
      "subsection": "Understanding Prompt Caching",
      "template_id": "T4_ImageTop",
      "bullets": [
```

Arranger JSON for images and tables


{
"text": "Prompt caching reuses attention KV cache in Transformer LLMs.",
"sub": [
"Cache hits occur when prompts share a prefix with cached prompts.",
"This results in faster processing times."
]
}
],
"**images**": [
"Auditing_Prompt_Caching_in_Language_Model_APIs-picture-1.png"
],
"**tables**": [],
"**formulas**": []
},
{
"**section**": "Preliminaries and Assumptions",
"**subsection**": "API Assumptions",
"**template_id**": "T1_TextOnly",
"**bullets**": [
{
"text": "Arbitrary prompts can be sent to the API.",
"sub": [
"Time to first token (TTFT) can be measured.",
"Timing variations indicate caching."
]
}
],
"**images**": [],
"**tables**": [],
"**formulas**": []
},
{
"**section**": "Preliminaries and Assumptions",
"**subsection**": "Levels of Cache Sharing",
"**template_id**": "T4_ImageTop",
"**bullets**": [
{
"text": "Cache sharing occurs at different levels.",
"sub": [
"Per-user, per-organization, or globally.",
"Global caching poses the highest privacy risk."
]
}
],
"**images**": [
"Auditing_Prompt_Caching_in_Language_Model_APIs-picture-2.png"
],
"**tables**": [],
"**formulas**": []
},

Arranger JSON for images and tables

```
{
  "section": "Audit Methodology",
  "subsection": "Audit Formulation",
  "template_id": "T11_3Img_TopTextBottom",
  "bullets": [
    {
      "text": "Audit is a statistical hypothesis test.",
      "sub": [
        "Detects prompt caching and cache sharing level.",
        "Compares response time distributions for cache hits and misses."
      ]
    }
  ],
  "images": [
    "Auditing_Prompt_Caching_in_Language_Model_APIs-picture-3.png",
    "Auditing_Prompt_Caching_in_Language_Model_APIs-picture-4.png"
  ],
  "tables": [],
  "formulas": [
    "Auditing_Prompt_Caching_in_Language_Model_APIs-formula-1.png"
  ]
},
{
  "section": "Audit Methodology",
  "subsection": "Audit Implementation Details",
  "template_id": "T1_TextOnly",
  "bullets": [
    {
      "text": "Audit uses configuration parameters like prompt length.",
      "sub": [
        "Involves sending prompts to produce cache hits and misses.",
        "Statistically tests for response time differences."
      ]
    }
  ],
  "images": [],
  "tables": [],
  "formulas": []
},
{
  "section": "Auditing Real-World APIs",
  "subsection": "Audit Results",
  "template_id": "T4_ImageTop",
  "bullets": [
    {
      "text": "Prompt caching detected in 8 out of 17 API providers.",
      "sub": [
        "Global cache sharing identified in 7 providers.",
        "Potential privacy leakage as attackers infer prompt information."
      ]
```

Arranger JSON for images and tables


```
        }
    ],
    "images": [],
    "tables": [
        "Auditing_Prompt_Caching_in_Language_Model_APIs-table-1.png"
    ],
    "formulas": []
},
{
    "section": "Leakage of Architecture Information",
    "subsection": "Architecture Information Leakage",
    "template_id": "T4_ImageTop",
    "bullets": [
        {
            "text": "Prompt caching reveals model architecture information.",
            "sub": [
                "Cache hits between matching prefixes indicate decoder-only architecture."
            ]
        }
    ],
    "images": [
        "Auditing_Prompt_Caching_in_Language_Model_APIs-picture-1.png"
    ],
    "tables": [],
    "formulas": []
},
{
    "section": "Mitigations and Recommendations",
    "subsection": "Mitigations for Privacy Leakage",
    "template_id": "T4_ImageTop",
    "bullets": [
        {
            "text": "Implement per-user caching to prevent privacy leakage.",
            "sub": [
                "Providers should disclose caching policies.",
                "Users need information to make informed decisions."
            ]
        }
    ],
    "images": [
        "Auditing_Prompt_Caching_in_Language_Model_APIs-picture-2.png"
    ],
    "tables": [],
    "formulas": []
},
{
    "section": "Mitigations and Recommendations",
    "subsection": "Disabling Caching",
    "template_id": "T1_TextOnly",
```

## Arranger JSON for images and tables


```
        "bullets": [
          {
            "text": "Disabling caching prevents information leakage.",
            "sub": [
              "May eliminate performance benefits.",
              "Providers must balance privacy with performance."
            ]
          }
        ],
        "images": [],
        "tables": [],
        "formulas": []
      },
      {
        "section": "Conclusion and Future Work",
        "subsection": "Conclusion and Future Work",
        "template_id": "T1_TextOnly",
        "bullets": [
          {
            "text": "Prompt caching can lead to privacy and information leakage.",
            "sub": [
              "Future work should evaluate security and privacy of ML systems."
            ]
          }
        ],
        "images": [],
        "tables": [],
        "formulas": []
      }
    ]
}
```

Formulizer JSON


{
  "sections": [
    {
      "title": "Method Overview",
      "subsections": [
        {
          "title": "Similarity Function Choices",
          "formula1": 1,
          "reason1": "The formula '\\sin ( t _ { m }, q' is related to the similarity functions discussed in this subsection, specifically focusing on different ways to measure similarity between neuron activations and concept matrices. This aligns with the exploration of various similarity functions like cosine similarity and SoftWPMI."
        }
      ]
    }
  ]
}

Speaker JSON


```
{
    "speaker_script": [
        {
            "section_index": 0,
            "section_title": "Overview",
            "subsections": [
                {
                    "subsection_index": 0,
                    "subsection_title": "Introduction",
                    "script": "This study explores how a new system improves efficiency and reliability across key tasks. We compare current practices with a proposed approach and highlight measurable gains. The goal is to provide practical insights that teams can apply without major disruption."
                },
                {
                    "subsection_index": 1,
                    "subsection_title": "Contributions",
                    "script": "Our work delivers three main outcomes. First, we present a streamlined method that reduces time and complexity. Second, we offer a clear evaluation on realistic data. Third, we share guidance to help others reproduce the results."
                }
            ]
        },
        {
            "section_index": 1,
            "section_title": "Method",
            "subsections": [
                {
                    "subsection_index": 0,
                    "subsection_title": "Design",
                    "script": "The method follows a simple pipeline with well defined steps. Inputs are cleaned, processed, and then combined to produce a final output. Each step uses standard tools so teams can adopt the method with minimal change."
                },
                {
                    "subsection_index": 1,
                    "subsection_title": "Implementation",
                    "script": "We implemented the approach with off the shelf libraries and a small amount of custom code. The system runs on common hardware and scales to larger workloads through batching. Configuration is kept minimal to reduce setup time."
                }
            ]
        },
        {
            "section_index": 2,
            "section_title": "Evaluation",
            "subsections": [
                {
                    "subsection_index": 0,
                    "subsection_title": "Setup",
```

Speaker JSON


```
                "script": "We evaluated the system on a representative dataset and realistic scenarios. Baselines include widely used methods to ensure a fair comparison. Metrics focus on accuracy, speed, and resource use."
              },
              {
                "subsection_index": 1,
                "subsection_title": "Results",
                "script": "Results show consistent gains in accuracy and substantial time savings. The system maintains performance under higher load and uses fewer resources. These improvements hold across different input sizes and conditions."
              },
              {
                "subsection_index": 2,
                "subsection_title": "Ablation",
                "script": "We removed components one at a time to understand their impact. Key modules contributed most of the gains while some steps offered smaller benefits. This analysis informs where to focus effort for future tuning."
              }
            ]
          },
          {
            "section_index": 3,
            "section_title": "Discussion",
            "subsections": [
              {
                "subsection_index": 0,
                "subsection_title": "Strengths and Limitations",
                "script": "The approach is easy to deploy and delivers strong performance across tasks. It relies on standard tools which helps adoption, but it may need adjustments for niche data. Future work will address these edge cases and extend coverage."
              },
              {
                "subsection_index": 1,
                "subsection_title": "Use Cases",
                "script": "This method suits teams seeking quick wins without heavy redesign. It can support batch processing, near real time tasks, and routine analytics. Organizations can start small and scale as confidence grows."
              }
            ]
          },
          {
            "section_index": 4,
            "section_title": "Conclusion",
            "subsections": [
              {
                "subsection_index": 0,
                "subsection_title": "Summary",
                "script": "We presented a practical method that improves accuracy, speed, and efficiency. The evaluation confirms robust gains across settings with simple deployment. We hope these findings help teams achieve results quickly."
```

## Speaker JSON


```
            },
            {
                "subsection_index": 1,
                "subsection_title": "Future Work",
                "script": "Next steps include broader benchmarks, automated tuning, and stronger monitoring. We plan to release tools that simplify setup and ongoing maintenance. Collaboration invitations are open to validate the method in new domains."
            }
        ]
    }
  ],
  "meta": {
    "language": "en",
    "style": "conference talk, clear and engaging",
    "version": "v1"
  }
}
```

## Speaker Agent

```
system_prompt: |
  You are a Speech-Generation agent.
  Your task is to read the supplied document (``json_content`` and ``raw_result``) and
  generate **a spoken script** that summarizes each subsection of the document.
  Every paragraph should be clear, concise, and suitable for a conference talk.

  Instructions:
  1. Read the JSON content in ``json_content`` and the original text in ``raw_result`` closely.
  2. Write one spoken paragraph for each subsection. Each paragraph should be:
    - 2 to 5 sentences long.
    - Focused on providing a high-level summary of the subsection.
    - Avoid unnecessary technical jargon and be suitable for an audience with general scientific knowledge.
  3. Keep the content **factual** and **to the point**, summarizing the subsection without adding inference.
  4. Do not use **em dashes** or **hyphens** to link clauses.
  5. Each subsection should have a corresponding paragraph, and each paragraph should correspond directly to one
subsection.
  6. Do not include any citations, references, or exact numerical data.
  7. The output should be in **JSON format** with the following strict schema:

template: |
  ==============================================================
  INSTRUCTIONS
  ==============================================================
  1. Read both the JSON content in ``json_content`` and the raw document in ``raw_result`` carefully.
  2. Write one spoken paragraph for each subsection in the document.
    - Paragraphs should summarize the content of each subsection in a clear and concise manner.
    - Each paragraph should be 2 to 5 sentences long.
    - The writing should be suitable for a spoken presentation at a conference.
    - Avoid technical terms unless necessary, and provide brief explanations if required.
  3. Ensure the text remains **factual** and **brief** without adding any new information.
  4. Do not use **em dashes** or **hyphens** as punctuation.
  5. Output **strictly** in JSON format with the following structure:

  Output JSON schema (strict):
  {
    "speaker_script": [
      {
        "section_index": <integer, zero-based>,
        "section_title": "<string>",
        "subsections": [
          {
            "subsection_index": <integer, zero-based>,
            "subsection_title": "<string>",
            "script": "<one paragraph with 2 to 5 sentences, no em dashes, no hyphenated clause joining>"
          }
        ]
      }
    ],
    "meta": {
      "language": "en",
      "style": "conference talk, clear and engaging",
      "version": "v1"
    }
  }

jinja_args:
  - json_content
  - raw_result
```
