# Supplementary material for: SlideGen: Collaborative Multimodal Agents for Scientific Slide Generation
Source: arXiv:2512.04529 source file (2026-08-22)
Supplement: Supplementary file 6 [file arrangerJSON.pdf]

## Arranger JSON for images and tables

```
{
  "slides": [
    {
      "section": "Introduction to Prompt Caching",
      "subsection": "Introduction to Prompt Caching",
      "template_id": "T4_ImageTop",
      "bullets": [
        {
          "text": "Prompt caching leads to data-dependent timing variations.",
          "sub": [
            "Cached prompts are processed faster than non-cached ones.",
            "This can result in side-channel timing attacks."
          ]
        },
        {
          "text": "Shared caches across users increase privacy risks.",
          "sub": [
            "If caches are shared, attackers can infer prompt information."
          ]
        }
      ],
      "images": [
        "Auditing_Prompt_Caching_in_Language_Model_APIs-picture-1.png"
      ],
      "tables": [],
      "formulas": []
    },
    {
      "section": "Introduction to Prompt Caching",
      "subsection": "Risks of Timing Attacks",
      "template_id": "T1_TextOnly",
      "bullets": [
        {
          "text": "Timing differences can be exploited by attackers.",
          "sub": [
            "Attackers can infer information about other users' prompts.",
            "Global cache sharing poses significant privacy concerns."
          ]
        }
      ],
      "images": [],
      "tables": [],
      "formulas": []
    },
    {
      "section": "Preliminaries and Assumptions",
      "subsection": "Understanding Prompt Caching",
      "template_id": "T4_ImageTop",
      "bullets": [
```

## Arranger JSON for images and tables

```
{
  "text": "Prompt caching reuses attention KV cache in Transformer LLMs.",
  "sub": [
    "Cache hits occur when prompts share a prefix with cached prompts.",
    "This results in faster processing times."
  ]
},
{
  "images": [
    "Auditing_Prompt_Caching_in_Language_Model_APIs-picture-1.png"
  ],
  "tables": [],
  "formulas": []
},
{
  "section": "Preliminaries and Assumptions",
  "subsection": "API Assumptions",
  "template_id": "T1_TextOnly",
  "bullets": [
    {
      "text": "Arbitrary prompts can be sent to the API.",
      "sub": [
        "Time to first token (TTFT) can be measured.",
        "Timing variations indicate caching."
      ]
    }
  ]
},
{
  "images": [],
  "tables": [],
  "formulas": []
},
{
  "section": "Preliminaries and Assumptions",
  "subsection": "Levels of Cache Sharing",
  "template_id": "T4_ImageTop",
  "bullets": [
    {
      "text": "Cache sharing occurs at different levels.",
      "sub": [
        "Per-user, per-organization, or globally.",
        "Global caching poses the highest privacy risk."
      ]
    }
  ]
},
{
  "images": [
    "Auditing_Prompt_Caching_in_Language_Model_APIs-picture-2.png"
  ],
  "tables": [],
  "formulas": []
},
}
```

## Arranger JSON for images and tables

```
{
  "section": "Audit Methodology",
  "subsection": "Audit Formulation",
  "template_id": "T11_3Img_TopTextBottom",
  "bullets": [
    {
      "text": "Audit is a statistical hypothesis test.",
      "sub": [
        "Detects prompt caching and cache sharing level.",
        "Compares response time distributions for cache hits and misses."
      ]
    }
  ],
  "images": [
    "Auditing_Prompt_Caching_in_Language_Model_APIs-picture-3.png",
    "Auditing_Prompt_Caching_in_Language_Model_APIs-picture-4.png"
  ],
  "tables": [],
  "formulas": [
    "Auditing_Prompt_Caching_in_Language_Model_APIs-formula-1.png"
  ]
},
{
  "section": "Audit Methodology",
  "subsection": "Audit Implementation Details",
  "template_id": "T1_TextOnly",
  "bullets": [
    {
      "text": "Audit uses configuration parameters like prompt length.",
      "sub": [
        "Involves sending prompts to produce cache hits and misses.",
        "Statistically tests for response time differences."
      ]
    }
  ],
  "images": [],
  "tables": [],
  "formulas": []
},
{
  "section": "Auditing Real-World APIs",
  "subsection": "Audit Results",
  "template_id": "T4_ImageTop",
  "bullets": [
    {
      "text": "Prompt caching detected in 8 out of 17 API providers.",
      "sub": [
        "Global cache sharing identified in 7 providers.",
        "Potential privacy leakage as attackers infer prompt information."
      ]
    }
  ]
}
```

## Arranger JSON for images and tables

```
    }
  ],
  "images": [],
  "tables": [
    "Auditing_Prompt_Caching_in_Language_Model_APIs-table-1.png"
  ],
  "formulas": []
},
{
  "section": "Leakage of Architecture Information",
  "subsection": "Architecture Information Leakage",
  "template_id": "T4_ImageTop",
  "bullets": [
    {
      "text": "Prompt caching reveals model architecture information.",
      "sub": [
        "Cache hits between matching prefixes indicate decoder-only architecture."
      ]
    }
  ],
  "images": [
    "Auditing_Prompt_Caching_in_Language_Model_APIs-picture-1.png"
  ],
  "tables": [],
  "formulas": []
},
{
  "section": "Mitigations and Recommendations",
  "subsection": "Mitigations for Privacy Leakage",
  "template_id": "T4_ImageTop",
  "bullets": [
    {
      "text": "Implement per-user caching to prevent privacy leakage.",
      "sub": [
        "Providers should disclose caching policies.",
        "Users need information to make informed decisions."
      ]
    }
  ],
  "images": [
    "Auditing_Prompt_Caching_in_Language_Model_APIs-picture-2.png"
  ],
  "tables": [],
  "formulas": []
},
{
  "section": "Mitigations and Recommendations",
  "subsection": "Disabling Caching",
  "template_id": "T1_TextOnly",
```

## Arranger JSON for images and tables

```
{
  "bullets": [
    {
      "text": "Disabling caching prevents information leakage.",
      "sub": [
        "May eliminate performance benefits.",
        "Providers must balance privacy with performance."
      ]
    }
  ],
  "images": [],
  "tables": [],
  "formulas": []
},
{
  "section": "Conclusion and Future Work",
  "subsection": "Conclusion and Future Work",
  "template_id": "T1_TextOnly",
  "bullets": [
    {
      "text": "Prompt caching can lead to privacy and information leakage.",
      "sub": [
        "Future work should evaluate security and privacy of ML systems."
      ]
    }
  ],
  "images": [],
  "tables": [],
  "formulas": []
}
]
```
