# Supplementary material for: SlideGen: Collaborative Multimodal Agents for Scientific Slide Generation
Source: arXiv:2512.04529 source file (2026-08-22)
Supplement: Supplementary file 7 [file mapper.pdf]

## Mapper JSON for images and tables

```
{
  "sections": [
    {
      "title": "Proposed Method: Multi-Turn Program Synthesis",
      "subsections": [
        {
          "title": "Multi-Turn Approach",
          "image1": 1,
          "reason": "Image 1 provides an illustrative example of the Multi-Turn Programming Benchmark, which aligns with the multi-turn approach described in this subsection."
        },
        {
          "title": "Advantages of Multi-Turn Synthesis",
          "table1": 3,
          "reasonT1": "Table 3 shows evaluation results on the Multi-Turn Programming Benchmark, directly related to the advantages of multi-turn synthesis discussed here."
        }
      ]
    },
    {
      "title": "Experiments and Evaluation",
      "subsections": [
        {
          "title": "Single-Turn Evaluation",
          "table1": 1,
          "reasonT1": "Table 1 presents evaluation results on the HumanEval benchmark, relevant to the single-turn evaluation discussed in this subsection."
        },
        {
          "title": "Multi-Turn Evaluation",
          "image1": 2,
          "reason": "Image 2 shows the difference in pass rates between single-turn and multi-turn formulations, which is pertinent to the multi-turn evaluation."
        }
      ]
    },
    {
      "title": "Results and Analysis",
      "subsections": [
        {
          "title": "Performance on Benchmarks",
          "table1": 4,
          "reasonT1": "Table 4 compares multi-turn and single-turn specifications, which is relevant to the performance analysis on benchmarks."
        }
      ]
    }
  ],
}
```

```
{
  "title": "Model Training and Datasets",
  "subsections": [
    {
      "title": "Datasets Used",
      "table1": 7,
      "reasonT1": "Table 5 provides statistics for training corpora, which is relevant to the
datasets used for training CODEGEN models."
    }
  ]
}
```
