# Supplementary material for: SlideGen: Collaborative Multimodal Agents for Scientific Slide Generation
Source: arXiv:2512.04529 source file (2026-08-22)
Supplement: Supplementary file 8 [file outlinerJSON.pdf]

## Outline JSON

```
{
  "metadata": {
    "title": "A Touch, Vision, and Language Dataset for Multimodal Alignment",
    "author": "Letian Fu; Gaurav Datta; Huang Huang; William Chung-Ho Panitch; Jaimyn Drake; Joseph Ortiz; Mustafa Mukadam; Mike Lambeta; Roberto Calandra; Ken Goldberg",
    "publish date": "2024",
    "organization": "UC Berkeley; Meta AI; TU Dresden"
  },
  "sections": [
    {
      "title": "Motivation: Why Integrate Touch With Vision And Language?",
      "subsections": [
        {
          "title": "Gaps In Multimodal Models",
          "content": "Most multimodal generative and alignment models focus on visual, textual, and sometimes audio or action signals, leaving tactile sensing underexplored. Yet touch captures material, texture, compliance, and force-related semantics vital for manipulation and human-like perception. A lack of open-vocabulary tactile-language data and difficulty synchronizing tactile with visual context impede progress. This work addresses scarce labels, subjective descriptions, and misalignment by proposing a dataset and models that align tactile, visual, and linguistic representations."
        },
        {
          "title": "Why Does This Matter?",
          "content": "Combining touch with vision and language can yield agents that more robustly infer material properties and contact states, improving open-vocabulary understanding and manipulation. The approach promises better generalization than vision-only models, enabling text-grounded tactile understanding and generation. It may benefit robotics, haptics research, and broader multimodal AI by providing a scalable path to tactile-language supervision via pseudo-labels."
        }
      ]
    },
    {
      "title": "Related Work And Limitations Of Existing Approaches",
      "subsections": [
        {
          "title": "Multimodal Encoders And Alignment",
          "content": "CLIP and derivatives align vision and language using contrastive learning; ImageBind extends to more modalities but primarily binds them through vision. Other works include masked multimodal pretraining and parameter-efficient alignment with LLMs. However, direct tactile-language alignment is typically absent, and tactile is often only bound to vision, limiting tactile semantic coverage."
        },
        {
          "title": "Tactile Perception And Datasets",
          "content": "Prior tactile-vision efforts address closed-set material or cloth classification and manipulation, often in lab settings, with limited vocabulary and diversity. Some datasets integrate audio or point clouds, but open-vocabulary tactile-language labels are missing. Concurrent efforts bind touch to vision without finetuning LLMs, leaving room for stronger tactile-language alignment
```

## Outline JSON

and generation."

```
    },
    {
      "title": "Training From Pseudo-Labels",
      "content": "Self-training and pseudo-labeling reduce annotation costs. Recent LLM/VLM pipelines use GPT-generated instruction data, but typically with matching input-output modalities. Here, vision-only GPT-4V generates tactile descriptions from images to supervise alignment with tactile data, expanding labeled coverage while acknowledging potential label noise."
    }
  ],
},
{
  "title": "Key Contributions Of This Work",
  "subsections": [
    {
      "title": "TVL Dataset: 44K Vision\u2013Tactile\u2013Language Triplets",
      "content": "A new dataset with 43,741 in-contact vision\u2013tactile pairs and open-vocabulary labels: 10% human-annotated (SSVTP) and 90% GPT-4V pseudo-labeled (HCT). The dataset spans in-the-wild settings, synchronized acquisition, and 254 unique tactile adjectives. A 99%/1% split is used with a human-labeled test set."
    },
    {
      "title": "Vision- And Language-Aligned Tactile Encoder",
      "content": "A tactile encoder trained via pairwise contrastive learning across tactile\u2013language, tactile\u2013vision, and vision\u2013language pairs, aligning tactile inputs directly to CLIP\u2019s latent space. Training strategies include inclusion of background (no-contact) frames labeled as \u2018background,\u2019 projector removal for vision/text, and randomized adjective subsets to improve robustness."
    },
    {
      "title": "TVL-LLaMA: Touch\u2013Vision\u2013Language Generation",
      "content": "A multimodal generation model finetuning LLaMA2-7B with TVL encoders to produce tactile descriptions from tactile and visual inputs. Two-stage training follows ImageBind-LLM style fusion, with additional instruction data (LLaVA CC3M, Alpaca, LLaVA 150K) to counter safety refusals and improve instruction-following."
    }
  ]
},
{
  "title": "Dataset: Collection, Cleaning, And Language Labeling",
  "subsections": [
    {
      "title": "Hardware And Synchronous Data Collection",
      "content": "A 3D-printed handheld rig integrates a DIGIT tactile sensor and a Logitech BRIO webcam to capture synchronized tactile and visual streams at 30 Hz during approach, contact, slide, and withdrawal trajectories. Five human collectors gathered 20 hours of diverse in-the-wild interactions ensuring the contact region remains in view, boosting variety and alignment fidelity."
    },
  ]
}
```

## Outline JSON

```
{
  "title": "Cleaning: Contact Versus No-Contact Frames",
  "content": "Using a pretrained tactile encoder, frames are categorized by cosine similarity to a background embedding; contact is flagged when similarity drops below 0.6. The final dataset includes 43,741 in-contact and 169,292 out-of-contact pairs. Contact frames are used primarily for training alignment and evaluation; a portion of no-contact frames aids generalization."
},
{
  "title": "Language Labeling: Human And GPT-4V Pseudo-Labels",
  "content": "SSVTP pairs are human-labeled using up to five adjectives drawn from a curated 400-word tactile vocabulary. HCT labels are generated by GPT-4V using both full and cropped images around the contact. Failures (e.g., occlusions, blur) are mitigated by labeling nearby frames within a trajectory or dropping unlabeled trajectories. Overall, 39,154 pseudo-labeled images are produced."
},
{
  "title": "Dataset Statistics And Split",
  "content": "SSVTP: 4,587 pairs; HCT: 39,154 in-contact and 169,292 no-contact pairs across 1,486 trajectories. A 99/1 train-test split is used; the test set (402 pairs) is human-labeled. GPT-4V averages 4.25 adjectives per item vs. 2.70 for humans, covering 254 distinct descriptors and yielding a long-tailed vocabulary distribution."
}
],
{
  "title": "Method Overview And Technical Design",
  "subsections": [
    {
      "title": "Contrastive Alignment Across All Modality Pairs",
      "content": "Unlike ImageBind\u2019s vision-centric binding, TVL optimizes InfoNCE across tactile\u2013language, tactile\u2013vision, and vision\u2013language. The tactile encoder (ViT-Tiny/Small/Base) is randomly initialized and projects to CLIP\u2019s latent space; vision/text use frozen OpenCLIP without additional projectors. Training shuffles and subsets language adjectives per sample for label diversity and includes 10% no-contact frames labeled \u2018background\u2019 to curb overfitting."
    },
    {
      "title": "Instruction Tuning With Multimodal Tokens",
      "content": "TVL-LLaMA follows ImageBind-LLM/LLaMA-Adapter fusion, averaging vision and tactile latents into a single token and using a zero-initialized gate and LoRA for efficient alignment. Pretraining uses LLaVA CC3M subset and TVL (empty tactile image for CC3M), followed by finetuning on TVL, Alpaca, and LLaVA 150K to improve instruction following and safety-guarded refusals."
    },
    {
      "title": "Prompting And Preprocessing Choices",
      "content": "Prompts are diversified for tactile description generation during fine-tuning; evaluation uses GPT-4 grading prompts with order randomization to reduce bias."
    }
  ]
}
```

## Outline JSON

Tactile preprocessing includes padding, resizing to 224x224, optional background subtraction, and normalization. Vision preprocessing uses CLIP statistics and tailored crops to keep sensor contact visible, matching GPT-4V labeling conditions."

```
    }
  ],
},
{
  "title": "Experiments, Datasets, And Evaluation Protocols",
  "subsections": [
    {
      "title": "Open-Vocabulary Cross-Modal Classification",
      "content": "On the human-labeled TVL test set (402-way), top-1/top-5 accuracy is computed for tactile\u2013vision and tactile\u2013language. To handle synonymy and order sensitivity in CLIP text embeddings, a synonym-expanded label set is built via GPT-4; cosine similarity thresholds define correctness. Vision\u2013text uses OpenCLIP scores. Baselines include SSVTP encoders and CLIP."
    },
    {
      "title": "TVL Benchmark For Tactile Description Generation",
      "content": "Given full image, cropped image, and tactile frame, models output up to five adjectives. GPT-4 scores responses against human labels from 1\u201310 with rationales. Models compared include GPT-4V, LLaVA variants, ViP-LLaVA, LLaMA-Adapter, BLIP-2, InstructBLIP, SSVTP-LLaMA, and TVL-LLaMA (Tiny/Small/Base). Statistical significance is assessed via paired t-tests."
    },
    {
      "title": "Additional Tasks And Ablations",
      "content": "A zero-shot binary object category test (fabric vs. plastic) illustrates downstream utility. Ablations analyze encoder size, disabling tactile\u2013text loss, modality removal, no-contact data mixing, prompt variants, background subtraction, training subsets (SSVTP vs. HCT vs. TVL), and freezing vs. finetuning the LLM. Overfitting to pseudo-labels and distribution shift between human and GPT-4V labels are examined."
    }
  ]
},
{
  "title": "Results And Comparative Analysis",
  "subsections": [
    {
      "title": "Classification Performance",
      "content": "TVL tactile encoders achieve strong tactile\u2013vision (up to 81.7% top-1) and tactile\u2013text (up to 36.7% top-1) accuracy on the TVL test set, outperforming SSVTP on in-the-wild data and surpassing OpenCLIP\u2019s vision\u2013text alignment for tactile semantics. Direct tactile\u2013text supervision is crucial; removing it reduces tactile\u2013text accuracy markedly."
    },
  ],
}
```

## Outline JSON

```
{
  "title": "TVL Benchmark: Generation Scores",
  "content": "TVL-LLaMA outperforms GPT-4V by at least 12% and open-source VLMs by larger margins, with significant p-values. Improvements hold across SSVTP (lab) and HCT (in-the-wild) subsets, showing benefits from limited human labels and extensive pseudo-labels. SSVTP-LLaMA, lacking tactile\u2013text pretraining, underperforms, underscoring the need for explicit tactile-language alignment."
},
{
  "title": "Ablation Insights And Sensitivity",
  "content": "Including all modality pair losses boosts alignment; background subtraction and limited no-contact data mitigate overfitting and improve downstream scores. Encoder size trades off robustness and overfitting to pseudo-labels. Prompt format has minor effects. Freezing the LLM can match finetuning in some settings, suggesting strong encoder alignment to language space."
}
],
{
  "title": "Limitations, Conclusion, And Future Directions",
  "subsections": [
    {
      "title": "Current Limitations",
      "content": "Vision-derived pseudo-labels may misdescribe tactile sensations when contact is occluded or ambiguous. Distribution shifts between GPT-4V pseudo-labels and human test labels can cause overfitting or evaluation gaps. Safety tuning in LLaMA2 required additional instruction data to avoid refusals. The vocabulary distribution is long-tailed with some noisy descriptors."
    },
    {
      "title": "Conclusion And Broader Impact",
      "content": "TVL provides a large-scale, synchronized vision\u2013tactile dataset with open-vocabulary labels, enabling a tactile encoder aligned with both vision and language and a TVL-LLaMA capable of generating tactile descriptions. Results demonstrate improved tactile-vision-language alignment and generation over strong baselines. The work advances embodied AI and robotic manipulation through richer multimodal grounding."
    },
    {
      "title": "Future Work",
      "content": "Scale human-labeled coverage, diversify environments and sensors, improve pseudo-label uncertainty handling, and explore richer task formulations (e.g., action-conditioned tactile reasoning). Investigate better fusion strategies beyond latent averaging, domain adaptation for occlusion or lighting, and extended downstream tasks such as open-world material and affordance understanding."
    }
  ]
}
]
```
